# Supplementary material for: Probabilistic $K$-mean with local alignment for clustering and motif discovery in functional data
Source: arXiv:1808.04773 ancillary file (2020-07-07)
Supplement: Supplementary file 1 [file paper_motifs_supplement.pdf]

# Supplementary material

# S1 Proofs

*Proof of Proposition 1.* We start considering the minimization of the functional (2) ignoring the constraint $\sum_{i=1}^{N} \hat{p}_{k,i} > 0$ for all $k$. In this case, the membership probability vectors $\mathbf{p}_i = [p_{1,i}, \ldots, p_{K,i}]$ related to different curves $\mathbf{x}_i$ vary independently and

$$\min_{\substack{p_{k,i}\in[0,1] \\ \sum_{k=1}^K p_{k,i}=1}} J_m(\mathbf{P}, \hat{\mathbf{S}}, \hat{\mathbf{v}}_1, \ldots, \hat{\mathbf{v}}_K) = \sum_{i=1}^{N} \min_{\substack{p_{k,i}\geq 0 \\ \sum_{k=1}^K p_{k,i}=1}} \sum_{k=1}^{K} (p_{k,i})^m d^2(\tilde{\mathbf{x}}_{i,\hat{s}_{k,i}}, \hat{\mathbf{v}}_k).$$

Hence the optimization problem is equivalent to $N$ independent minimizations, for any $i = 1, \ldots, N$, of the functions $f_{m,i} : \mathbb{R}^K \longrightarrow \mathbb{R}$, $\mathbf{p}_i \longmapsto \sum_{k=1}^{K} (p_{k,i})^m d^2(\tilde{\mathbf{x}}_{i,\hat{s}_{k,i}}, \hat{\mathbf{v}}_k)$ subject to the constraints $p_{k,i} \geq 0$ and $\sum_{k=1}^{K} p_{k,i} = 1$.

For $i \notin R$, $f_{m,i}$ with constraints $p_{k,i} \geq 0$ and $\sum_{k=1}^{K} p_{k,i} = 1$ is minimized by $\hat{\mathbf{p}}_i$ if and only if it satisfies (4). In particular, $f_{m,i}(\hat{\mathbf{p}}_i) = 0$.

For $i \in R$, we employ Karush-Kuhn-Tucker conditions on $f_{m,i}$ with constraints $g_k(\mathbf{p}_i) = -p_{k,i} \leq 0$ for all $k$ and $h(\mathbf{p}_i) = \sum_{k=1}^{K} p_{k,i} - 1 = 0$. Regularity conditions are satisfied ($f_{m,i}$, $g_k$ and $h$ are continuously differentiable, $g_k$ and $h$ are affine functions) and the Lagrangian associated to the optimization problem is given by $\mathcal{L}(\mathbf{p}_i, \lambda, \mu) = f_{m,i}(\mathbf{p}_i) - \sum_{k=1}^{K} \lambda_k p_{k,i} + \mu \left(\sum_{k=1}^{K} p_{k,i} - 1\right)$. If $\hat{\mathbf{p}}_i$ is a constrained minimizer of $f_{m,i}$ then there exist constants $\hat{\lambda}$ and $\hat{\mu}$, with $(\lambda, \hat{\mu}) \neq \mathbf{0}$, such that the following conditions hold:

$$\nabla f_{m,i}(\mathbf{p}_i) - \sum_{k=1}^{K} \hat{\lambda}_k \nabla p_{k,i} + \hat{\mu} \nabla \left(\sum_{k=1}^{K} p_{k,i} - 1\right)\Bigg|_{\mathbf{p}_i=\hat{\mathbf{p}}_i} = \mathbf{0}, \tag{19}$$

$$\hat{\lambda}_k \hat{p}_{k,i} = 0 \qquad k = 1, \ldots, K, \tag{20}$$

$$\hat{\lambda}_k \geq 0 \qquad k = 1, \ldots, K. \tag{21}$$

Condition (19) implies $\frac{\partial f_{m,i}}{\partial p_{k,i}}(\hat{\mathbf{p}}_i) - \hat{\lambda}_k + \hat{\mu} = 0$ for each $k$, and hence

$$\hat{p}_{k,i} = \left(\frac{\hat{\lambda}_k - \hat{\mu}}{m\, d^2\left(\tilde{\mathbf{x}}_{i,\hat{s}_{k,i}}, \hat{\mathbf{v}}_k\right)}\right)^{\frac{1}{m-1}}.$$

From $\hat{p}_{k,i} \geq 0$ follows $\hat{\lambda}_k \geq \hat{\mu}$ for all $k$. Suppose there exists $l$ such that $\hat{\lambda}_l > 0$. Then condition (20) implies $\hat{p}_{l,i} = 0$, hence $\hat{\lambda}_l = \hat{\mu}$. Then, for all $k$, we obtain $0 < \hat{\lambda}_l = \hat{\mu} \leq \hat{\lambda}_k$ and hence, from condition (20), $\hat{p}_{k,i} = 0$. This solution is not admissible because it does not respect the constraint $\sum_{k=1}^{K} p_{k,i} = 1$, hence we must have $\hat{\lambda} = \mathbf{0}$, $\hat{\mu} < 0$ and $\hat{p}_{k,i} = \left(\frac{-\hat{\mu}}{m\, d^2\left(\tilde{\mathbf{x}}_{i,\hat{s}_{k,i}}, \hat{\mathbf{v}}_k\right)}\right)^{\frac{1}{m-1}}$, $k = 1, \ldots, K$. In order to compute the value of $\hat{\mu}$ we use the constraint $\sum_{k=1}^{K} p_{k,i} = 1$, obtaining

$$\hat{p}_{k,i} = \left[\sum_{l=1}^{K} \left(\frac{d^2\left(\tilde{\mathbf{x}}_{i,\hat{s}_{k,i}}, \hat{\mathbf{v}}_k\right)}{d^2\left(\tilde{\mathbf{x}}_{i,\hat{s}_{l,i}}, \hat{\mathbf{v}}_l\right)}\right)^{\frac{1}{m-1}}\right]^{-1} \qquad k = 1, \ldots, K.$$

To show that the previous equation is also sufficient for $\hat{\mathbf{p}}_i$ to be a constrained minimizer of $f_{m,i}$, we observe that $f_{m,i}$, $g_k$ and $h$ are twice continuously differentiable and we consider the Hessian matrix $H_{\mathcal{L}} = \left[\frac{\partial^2 \mathcal{L}_{m,i}}{\partial p_{l,i} p_{k,i}}\right]$ of the Lagrangian. For $l \neq k$ we have $\frac{\partial^2 \mathcal{L}_{m,i}}{\partial p_{l,i} p_{k,i}} = 0$, while for $l = k$ we have $\frac{\partial^2 \mathcal{L}_{m,i}}{\partial^2 p_{k,i}}(\mathbf{p}_i, \lambda, \mu) = m(m-1)(p_{k,i})^{m-2} d^2\left(\tilde{\mathbf{x}}_{i,\hat{s}_{k,i}}, \hat{\mathbf{v}}_k\right)$. The diagonal matrix $H_{\mathcal{L}}$ is a positive definite matrix in the point $(\hat{\mathbf{p}}_i, \hat{\lambda}, \hat{\mu})$ that satisfies the first-order Karush-Kuhn-Tucker conditions (since $m > 1$ and $\hat{p}_{k,i} > 0$), hence $\hat{\mathbf{p}}_i$ is a strict local minimizer of $f_{m,i}$.

The set $\left\{\mathbf{p}_i \in \mathbb{R}^K \mid p_{k,i} \in [0,1], \sum_{k=1}^K p_{k,i} = 1\right\}$ is convex and the function $f_{m,i}$ is strictly convex (since $m > 1$ and $d(\tilde{\mathbf{x}}_{i,\hat{s}_{k,i}}, \hat{\mathbf{v}}_k)) > 0$ for all $k$), hence the local minimizer $\hat{\mathbf{p}}_i$ is actually the unique global minimizer of $f_{m,i}$.

Finally, the hypothesis $|R| \geq K$ guarantees that the solution $\hat{\mathbf{P}}$ defined by (3)-(4) satisfy the constraint $\sum_{i=1}^N \hat{p}_{k,i} > 0$ for all $k$. □

*Proof of Proposition 2.* Since the contribute of each cluster $k$ to the functional (6) is independent from the contributes of other clusters, we have

$$\min_{\mathbf{v}_1,\ldots,\mathbf{v}_K} J_m(\hat{\mathbf{P}}, \hat{\mathbf{S}}, \mathbf{v}_1, \ldots, \mathbf{v}_K) = \sum_{k=1}^K \min_{\mathbf{v}_1,\ldots,\mathbf{v}_K} \sum_{i=1}^N (\hat{p}_{k,i})^m d_\alpha^2\left(\tilde{\mathbf{x}}_{i,\hat{s}_{k,i}}, \mathbf{v}_k\right).$$

Hence we can solve $K$ independent optimization problems. In particular, for each cluster $k$ we minimize $g_{m,k} : V_k \longrightarrow \mathbb{R}$, $\mathbf{v}_k \longmapsto \sum_{i=1}^N (\hat{p}_{k,i})^m d_\alpha^2\left(\tilde{\mathbf{x}}_{i,\hat{s}_{k,i}}, \mathbf{v}_k\right)$. Let $\hat{\mathbf{v}}_k, \varphi \in V_k$ fixed and define $g : \mathbb{R} \longrightarrow \mathbb{R}$, that maps $u \longmapsto g_{m,k}(\hat{\mathbf{v}}_k + u\varphi) = \sum_{i=1}^N (\hat{p}_{k,i})^m d_\alpha^2\left(\tilde{\mathbf{x}}_{i,\hat{s}_{k,i}}, \hat{\mathbf{v}}_k + u\varphi\right)$. The function $g_{m,k}$ has a minimum in $\mathbf{v}_k = \hat{\mathbf{v}}_k$ if and only if $g$ has a minimum in $u = 0$. A necessary condition is $g'(0) = 0$, that implies $\frac{dg_{m,k}}{du}(\hat{\mathbf{v}}_k + u\varphi)\Big|_{u=0} = 0$ for all $\varphi \in V_k$. For every $\alpha \in [0,1)$, $d_\alpha$ is the distance induced by the following inner product in $V_k$:

$$\langle \mathbf{y}_1, \mathbf{y}_2 \rangle_\alpha = \frac{1}{d} \sum_{j=1}^d \frac{w_j}{c_k} \int_0^{c_k} \left[(1-\alpha) y_1^{(j)}(t) y_2^{(j)}(t) + \alpha y_1'^{(j)}(t) y_2'^{(j)}(t)\right] \mathrm{d}t. \tag{22}$$

For $\alpha = 1$, (22) satisfies all the inner product properties in $V_k$, with the exception that $\langle \mathbf{y}, \mathbf{y} \rangle_1 = 0$ only implies $\mathbf{y} = \mathbf{const}$ a.e. in $(0, c_k)$; $d_1$ is its induced semi-distance. Using this notation, we obtain

$$\begin{aligned} 0 &= \sum_{i=1}^N (\hat{p}_{k,i})^m \frac{d}{du}\left[\langle \tilde{\mathbf{x}}_{i,\hat{s}_{k,i}} - \hat{\mathbf{v}}_k, \tilde{\mathbf{x}}_{i,\hat{s}_{k,i}} - \hat{\mathbf{v}}_k \rangle_\alpha\right. \\ &= -2 \langle \sum_{i=1}^N (\hat{p}_{k,i})^m \left(\tilde{\mathbf{x}}_{i,\hat{s}_{k,i}} - \hat{\mathbf{v}}_k\right), \varphi \rangle_\alpha \end{aligned}$$

for every $\varphi \in V_k$. In particular, we can choose $\varphi = \sum_{i=1}^N (\hat{p}_{k,i})^m \left(\tilde{\mathbf{x}}_{i,\hat{s}_{k,i}} - \hat{\mathbf{v}}_k\right)$, obtaining

$$\langle \sum_{i=1}^N (\hat{p}_{k,i})^m \left(\tilde{\mathbf{x}}_{i,\hat{s}_{k,i}} - \hat{\mathbf{v}}_k\right), \sum_{i=1}^N (\hat{p}_{k,i})^m \left(\tilde{\mathbf{x}}_{i,\hat{s}_{k,i}} - \hat{\mathbf{v}}_k\right) \rangle_\alpha = 0. \tag{23}$$

If $\alpha \neq 1$, (23) implies $\sum_{i=1}^{N} (\hat{p}_{k,i})^m \left(\tilde{\mathbf{x}}_{i,\hat{s}_{k,i}} - \hat{\mathbf{v}}_k\right) = \mathbf{0}$ a.e. in $(0, c_k)$. Using the fact that $\sum_{i=1}^{N} \hat{p}_{k,i} > 0$ (non-degenerate clusters) we obtain

$$\hat{\mathbf{v}}_k = \frac{\displaystyle\sum_{i=1}^{N} (\hat{p}_{k,i})^m \tilde{\mathbf{x}}_{i,\hat{s}_{k,i}}}{\displaystyle\sum_{i=1}^{N} (\hat{p}_{k,i})^m} \qquad \text{a.e. in } (0, c_k).$$

If $\alpha = 1$, (23) implies $\sum_{i=1}^{N} (\hat{p}_{k,i})^m \left(\tilde{\mathbf{x}}_{i,\hat{s}_{k,i}} - \hat{\mathbf{v}}_k\right) = \mathbf{const}$ a.e. in $(0, c_k)$. Hence we have

$$\hat{\mathbf{v}}_k = \frac{\displaystyle\sum_{i=1}^{N} (\hat{p}_{k,i})^m \tilde{\mathbf{x}}_{i,\hat{s}_{k,i}}}{\displaystyle\sum_{i=1}^{N} (\hat{p}_{k,i})^m} + \mathbf{const} \qquad \text{a.e. in } (0, c_k).$$

To show the sufficiency of the previous equation for $\hat{\mathbf{v}}_k$ to be minimizer, we compute the second-order derivative of $g$: $g''(u) = 2 \sum_{i=1}^{N} (\hat{p}_{k,i})^m \langle \varphi, \varphi \rangle_\alpha$. Since $\sum_{i=1}^{N} \hat{p}_{k,i} > 0$, we have $g''(u) > 0$. Hence $u = 0$ is a strict local minimizer of $g$ and $\hat{\mathbf{v}}_k$ is a strict local minimizer of $g_{m,k}$.

The constraint $\sum_{i=1}^{N} \hat{p}_{k,i} > 0$ implies also that the function $g_{m,k}$ is strictly convex on $V_k$, hence the local minimizer $\hat{\mathbf{v}}_k$ is actually the unique global minimizer of $g_{m,k}$. □

*Proof of Lemma 3.* The functions $t \mapsto t + s_{k,i}$, $y \mapsto y^m$, and $d$ are continuous. The functional $J_m$ is the sum of products of compositions of continuous functions, hence it is continuous. □

*Proof of Theorem 4.* Let $\mathbf{y}^{(it-1)} = \left(\mathbf{P}^{(it-1)}, \mathbf{S}^{(it-1)}, \mathbf{v}_1^{(it-1)}, \ldots, \mathbf{v}_K^{(it-1)}\right) \in Y$. We have $\mathbf{y}^{(it)} \in T_m\left(\mathbf{y}^{(it-1)}\right)$, hence $\mathbf{v}_1^{(it)}, \ldots, \mathbf{v}_K^{(it)}$ are computed using equation (7). Hence from Proposition 2 follows

$$J_m\left(\mathbf{P}^{(it-1)}, \mathbf{S}^{(it-1)}, \mathbf{v}_1^{(it)}, \ldots, \mathbf{v}_K^{(it)}\right) \leq J_m\left(\mathbf{P}^{(it-1)}, \mathbf{S}^{(it-1)}, \mathbf{v}_1^{(it-1)}, \ldots, \mathbf{v}_K^{(it-1)}\right).$$

Similarly, $\mathbf{S}^{(it)}$ is selected in order to minimize the distances $d\left(\tilde{\mathbf{x}}_{i,s}, \mathbf{v}_k^{(it)}\right)$, so

$$J_m\left(\mathbf{P}^{(it-1)}, \mathbf{S}^{(it)}, \mathbf{v}_1^{(it)}, \ldots, \mathbf{v}_K^{(it)}\right) \leq J_m\left(\mathbf{P}^{(it-1)}, \mathbf{S}^{(it-1)}, \mathbf{v}_1^{(it)}, \ldots, \mathbf{v}_K^{(it)}\right).$$

Finally, $\mathbf{P}^{(it)}$ is computed using equations (3)-(4), hence from Preposition 1 we have

$$J_m\left(\mathbf{P}^{(it)}, \mathbf{S}^{(it)}, \mathbf{v}_1^{(it)}, \ldots, \mathbf{v}_K^{(it)}\right) \leq J_m\left(\mathbf{P}^{(it-1)}, \mathbf{S}^{(it)}, \mathbf{v}_1^{(it)}, \ldots, \mathbf{v}_K^{(it)}\right).$$

Combining the previous three equations we obtain (10).

Suppose now that $\mathbf{y}^{(it-1)} \notin \Omega$. If (13) does not hold for $\mathbf{y}^{(it-1)}$, then there exist $\mathbf{v}_k \in V_k$ with $\mathbf{v}_k \neq \mathbf{v}_k^{(it-1)}$ such that

$$J_m\left(\mathbf{P}^{(it-1)}, \mathbf{S}^{(it-1)}, \mathbf{v}_1^{(it-1)}, \ldots, \mathbf{v}_K^{(it-1)}\right) \geq J_m\left(\mathbf{P}^{(it-1)}, \mathbf{S}^{(it-1)}, \mathbf{v}_1, \ldots, \mathbf{v}_K\right)$$

and by Proposition 2 we know that $J_m(\mathbf{P}^{(it-1)}, \mathbf{S}^{(it-1)}, \cdot)$ has a unique global minimizer, hence

$$J_m\left(\mathbf{P}^{(it-1)}, \mathbf{S}^{(it-1)}, \mathbf{v}_1^{(it)}, \ldots, \mathbf{v}_K^{(it)}\right) < J_m\left(\mathbf{P}^{(it-1)}, \mathbf{S}^{(it-1)}, \mathbf{v}_1^{(it-1)}, \ldots, \mathbf{v}_K^{(it-1)}\right).$$

If $\mathbf{y}^{(it-1)}$ satisfies (13) but not (12), then $\mathbf{v}_k^{(it)} = \mathbf{v}_k^{(it-1)}$ and there exists $\mathbf{S} \in \mathbb{R}^{(K,N)}$ such that

$$J_m\left(\mathbf{P}^{(it-1)}, \mathbf{S}^{(it-1)}, \mathbf{v}_1^{(it)}, \ldots, \mathbf{v}_K^{(it)}\right) > J_m\left(\mathbf{P}^{(it-1)}, \mathbf{S}, \mathbf{v}_1^{(it)}, \ldots, \mathbf{v}_K^{(it)}\right).$$

Since $\mathbf{S}^{(it)}$ minimizes $d\left(\tilde{\mathbf{x}}_{i,s}, \mathbf{v}_k^{(it)}\right)$ we have that

$$J_m\left(\mathbf{P}^{(it-1)}, \mathbf{S}^{(it)}, \mathbf{v}_1^{(it)}, \ldots, \mathbf{v}_K^{(it)}\right) < J_m\left(\mathbf{P}^{(it-1)}, \mathbf{S}^{(it-1)}, \mathbf{v}_1^{(it)}, \ldots, \mathbf{v}_K^{(it)}\right).$$

Finally, if $\mathbf{y}^{(it-1)}$ satisfies (12) and (13), but not (11), we have that $\mathbf{v}_k^{(it)} = \mathbf{v}_k^{(it-1)}$ and there exists $\mathbf{P} \in [0,1]^{K,N}$, with $\sum_{k=1}^{K} p_{k,i} = 1$ and $\sum_{i=1}^{N} p_{k,i} > 0$, such that

$$J_m\left(\mathbf{P}^{(it-1)}, \mathbf{S}^{(it-1)}, \mathbf{v}_1^{(it)}, \ldots, \mathbf{v}_K^{(it)}\right) > J_m\left(\mathbf{P}, \mathbf{S}^{(it-1)}, \mathbf{v}_1^{(it)}, \ldots, \mathbf{v}_K^{(it)}\right).$$

Then from Proposition 1 and equation (12) follows that

$$\begin{aligned} J_m\left(\mathbf{P}^{(it)}, \mathbf{S}^{(it-1)}, \mathbf{v}_1^{(it)}, \ldots, \mathbf{v}_K^{(it)}\right) &< J_m\left(\mathbf{P}^{(it-1)}, \mathbf{S}^{(it-1)}, \mathbf{v}_1^{(it)}, \ldots, \mathbf{v}_K^{(it)}\right) \\ &\leq J_m\left(\mathbf{P}^{(it-1)}, \mathbf{S}^{(it)}, \mathbf{v}_1^{(it)}, \ldots, \mathbf{v}_K^{(it)}\right). \end{aligned}$$

The matrix $\mathbf{S}^{(it)}$ minimizes $d\left(\tilde{\mathbf{x}}_{i,s}, \mathbf{v}_k^{(it)}\right)$ and does not depend on $\mathbf{P}$, so we have

$$J_m\left(\mathbf{P}^{(it)}, \mathbf{S}^{(it)}, \mathbf{v}_1^{(it)}, \ldots, \mathbf{v}_K^{(it)}\right) \leq J_m\left(\mathbf{P}^{(it)}, \mathbf{S}^{(it-1)}, \mathbf{v}_1^{(it)}, \ldots, \mathbf{v}_K^{(it)}\right).$$

As a consequence

$$J_m\left(\mathbf{P}^{(it)}, \mathbf{S}^{(it)}, \mathbf{v}_1^{(it)}, \ldots, \mathbf{v}_K^{(it)}\right) < J_m\left(\mathbf{P}^{(it-1)}, \mathbf{S}^{(it)}, \mathbf{v}_1^{(it)}, \ldots, \mathbf{v}_K^{(it)}\right).$$

□

# S2 Functional motif discovery post-processing

Given the set of candidate motifs – obtained from multiple runs of probKMA and filtered based on generalized silhouette indices and number of occurrences – we propose the following implementation for the post-processing steps. The goal is to merge similar candidate motifs and locate all instances of the final set of functional motifs (see Section 3).

1. Compute all pairwise distances between candidate motifs;

2. Perform hierarchical clustering with average linkage of candidate motifs, using their pairwise distances;

3. Determine a global radius $R_{all}$ based on the minimum distances between all candidate motifs and all curves;

4. Cut the hierarchical clustering dendrogram at height $2R_{all}$, obtaining $M$ groups of similar motifs;

5. For each group $m = 1, \dots, M$:

   a. Determine a group-specific radius $R_m$ based on the minimum distances between the motifs of group $m$ and all curves;

   b. For each motif in group $m$

      - Find the curves containing the motif, i.e. the curves with distance $\leq R_m$ from the motif;
      - Approximate the number of occurrences in the curves (portions of curves with distance $\leq R_m$ from the motif), counting the number of curves containing the motif;
      - Approximate the average within-motif distance (average distance between the motif and its occurrences in the curves) with the average distance between the motif and the curves containing it;

   c. Select a very small number of motifs based on the approximate number of occurrences, the approximate radius and the motif length;

6. Find all occurrences of the selected motifs (portions of curves with distance $\leq R_m$ from the motif).

Pairwise distances between candidate motifs in step 1 are computed according to the same distance employed by probKMA, allowing alignment between each pair of motifs but requiring a minimum overlap, defined as a percentage of the shortest motif in each pair (default choice 60%).

During the last iteration of probKMA algorithm (and in particular in step iii) we compute the minimum distances between each motif and all curves. Moreover, the curves are divided in two groups: the ones that contain the motif, and the ones that do not contain it (cluster cleaning step, see Subsection 2.4). In steps 3 and 5a of the post-processing we utilize this piece of information in order to compute the radii $R_{all}$ and $R_m$ (see Fig. S1). In particular, we employ $k$-nearest neighbors to select the distance that "best discriminate" the group of distances between each motif and the curves that contain it (group 1), from the group of distances between each motif and the curves that do not contain it (group 0). This distance is selected based on the posterior probability of the $k$-nearest neighbors classifier (i.e. the percentage of votes for one group). The advantage of using a non-parametric classifier such as $k$-nearest neighbors is that we do not need any assumption on the distribution of distances in the two groups. However, it is important to observe that the resolution of the posterior depends on the number of neighbor used ($k = 1$ corresponds to probability of 0 and 1, $k = 2$ to 0, 0.5 and 1 and so on). In addition, the posterior probability of the $k$-nearest neighbors

classifier can be not decreasing: for intermediate distances between the two groups we can have a distance classified as group 0, then a distance classified as group 1, and then again a distance classified as group 0. In order to be conservative in defining group 1, we select the smallest distance at which the posterior probability of belonging to group 1 is smaller than a given threshold. Regarding the selection of $k$, with very small $k$ the algorithm is very fast but give very noisy results, while larger $k$ create more stable results but take much more computational time. Our default choice is $k = 3$ and threshold 0.5 for the posterior probability.

Selection of motifs in each group $m$ (step 5c, Fig. S2) is done maximizing the approximate number of occurrences while simultaneously minimizing the approximate average within-motif distance. In particular, we order the motifs based on the sum of their ranks in each of the two dimension, and we select the top one. If other motifs in the same group have length very different from the selected one, we can allow the procedure to select them too (by default, we select only the top motif in each group). The idea of using approximate metrics (step 5b, Figs. S2c and S2f) permits to avoid finding all occurrences for all motifs, since this would be computationally expensive.

Step 6 represents a motif search step, that is needed in order to locate all occurrences of the selected motifs, i.e. all portions of curves with distance $\leq R_m$ from each motif (with $R_m$ the group-specific radius for that motif). We observe that two overlapping portions of curves tend to be quite similar. Hence, if a portion of curve matches a particular motif, the portion of curve that begins and ends immediately at its left/right is likely to match the same motif too. In order to avoid counting multiple times the same motif occurrence, we require that two occurrences of the same motif are well separated (analogously to Lin et al., 2002). In

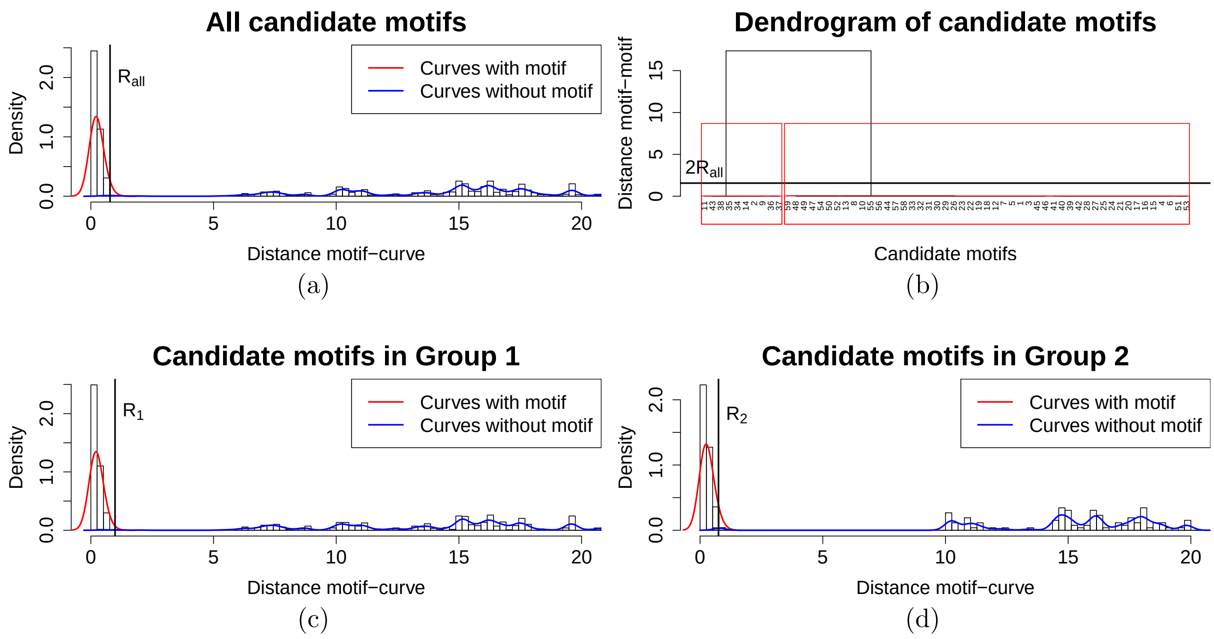


Figure S1: Example of post-processing, data from first simulation scenario in Subsection 4.2, $l = 200$, $\sigma = 1$. (a) Selection of a global radius $R_{all}$ (step 3); (b) Hierarchical clustering dendrogram cut at height $2R_{all}$ (step 4); (c)-(d) Selection of a group-specific radius $R_m$ in each of the two groups (step 5a).

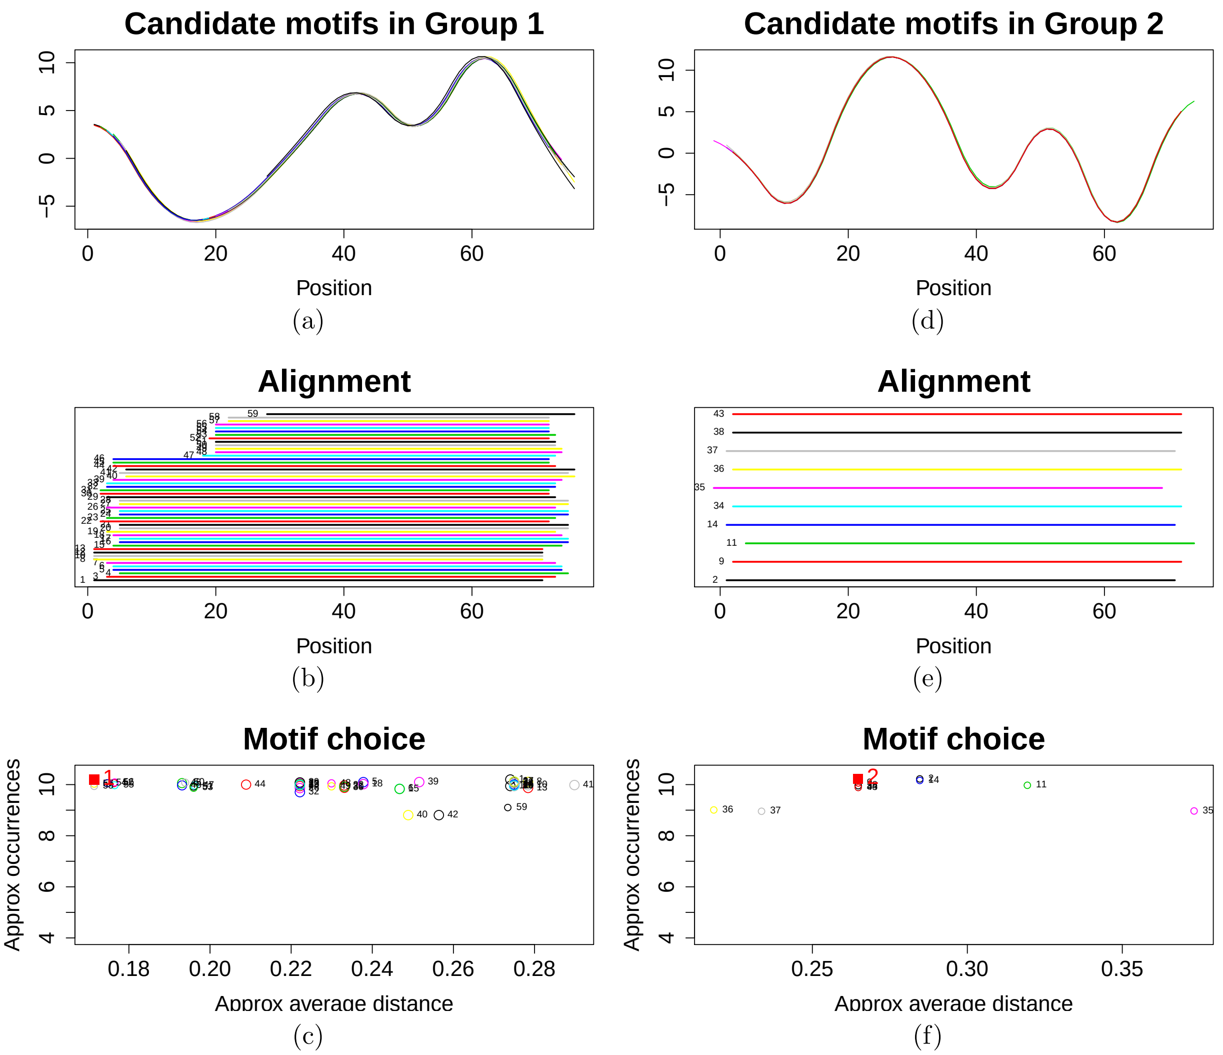


Figure S2: Example of post-processing, data from first simulation scenario in Subsection 4.2, $l = 200$, $\sigma = 1$. (a) Aligned candidate motifs in Group 1; (b) Alignment of candidate motifs in Group 1; (c) Approximate average within-motif distance vs approximate number of occurrences, for motifs in Group 1 (step 5b). Circle size is proportional to motif length. A red square indicates selected motif (step 5c); (d)-(f) Analogous plots for motifs in Group 2.

particular, let $\mathbf{v}_m$ be a selected motif that matches a curve $\mathbf{x}$ in two portions corresponding to the shifts $s_1 < s_2$, i.e. $d(\tilde{\mathbf{x}}_{s_1}, \mathbf{v}_m) \leq R_m$ and $d(\tilde{\mathbf{x}}_{s_2}, \mathbf{v}_m) \leq R_m$. In order to count both occurrences, we ask that there exists a shift $s \in (s_1, s_2)$ such that $d(\tilde{\mathbf{x}}_s, \mathbf{v}_m) > R_m$. Among all the $s \in (s_l, s_r)$ such that $d(\tilde{\mathbf{x}}_s, \mathbf{v}_m) \leq R_m$, with $d(\tilde{\mathbf{x}}_{s_l}, \mathbf{v}_m) > R_m$ and $d(\tilde{\mathbf{x}}_{s_r}, \mathbf{v}_m) > R_m$, we select as motif occurrence the portion corresponding to the shift that minimizes $d(\tilde{\mathbf{x}}_s, \mathbf{v}_m)$.

# S3 Simulations: additional figures and results

## S3.1 Functional motif discovery in curves with different lengths and motifs with different noise levels

Here we report additional information related to simulations in Subsection 4.2.

Figs. S3 and S4 show the two functional motifs and the 12 aligned occurrences of each, as well as the 20 curves embedding occurrences of the two motifs, for curve length $l = 200$ and noise levels $\sigma = 0.1, 0.5, 1, 2$, in simulation scenario (1). Figs. S5, S6 and S7 show the performance of our probKMA-based functional motif discovery for different levels of noise and curve lengths $l = 300, 400, 500$, respectively (results for curve length $l = 200$ are shown in Fig. 2). Analogous information for simulation scenario (2) are showed in Figs. S8-S13.

In simulation scenario (1), we employ Sobolev-like distance $d_{0.5}$ to measure similarities between pieces of curves, while in simulation scenario (2) we use the $L^2$-like pseudo-distance $d_1$ on the weak derivative. In both cases, probKMA is run for $K = 2, 3$, minimum motif lengths $c = 40, 50, 60$ and 20 random initializations for each $(K, c)$ pair. The same initializations (i.e. the same initial membership matrix $\mathbf{P}^{(0)}$ and shift matrix $\mathbf{S}^{(0)}$) are employed for all $l$ and $\sigma$ combinations. Weighting "fuzziness" parameter is fixed to be $m = 2$. ProbKMA iterations are stopped when the global Bhattacharyya distance $BC_{\max} = \max_{k=1,\ldots,K} BC_k$ is less then or equal to $10^{-8}$. Maximum motif length is set to 70. Elongation step (see Subsection 2.3) is performed at every iteration, when $BC_{\max} \leq 10^{-3}$; each center is elongated up to 50% of its length in either directions, requiring that the relative objective function $J_{m,k}$ increase is less than 5% (i.e. $(J_{m,k,\text{elong}} - J_{m,k})/J_{m,k} < 0.05$). Cleaning step (see Subsection 2.4) is performed every 50 iterations, when $BC_{\max} \leq 10^{-4}$. Candidate motifs that belong to less than 5 curves, as well as the ones with an average cluster silhouette index lower than the $90^{th}$ percentile of all overall average silhouette indices, are filtered out (see Section 3). Post-processing is performed with default values (see Section S2).

Fig. S14 shows aligned occurrences of functional motifs (for curve length $l = 200$ and level of noise $\sigma = 1$), for 10 different pairs of functional motifs and set of curves in simulation scenario (1). Summary results of 10 replications of functional motif discovery for each of these 10 datasets are shown in Fig. S15. Finally, Figs. S16-S17 show the corresponding plots in simulation scenario (2), while Fig. S18 shows the number of motifs discovered in the 10 replications of functional motif discovery, for the 10 simulations in both scenarios.

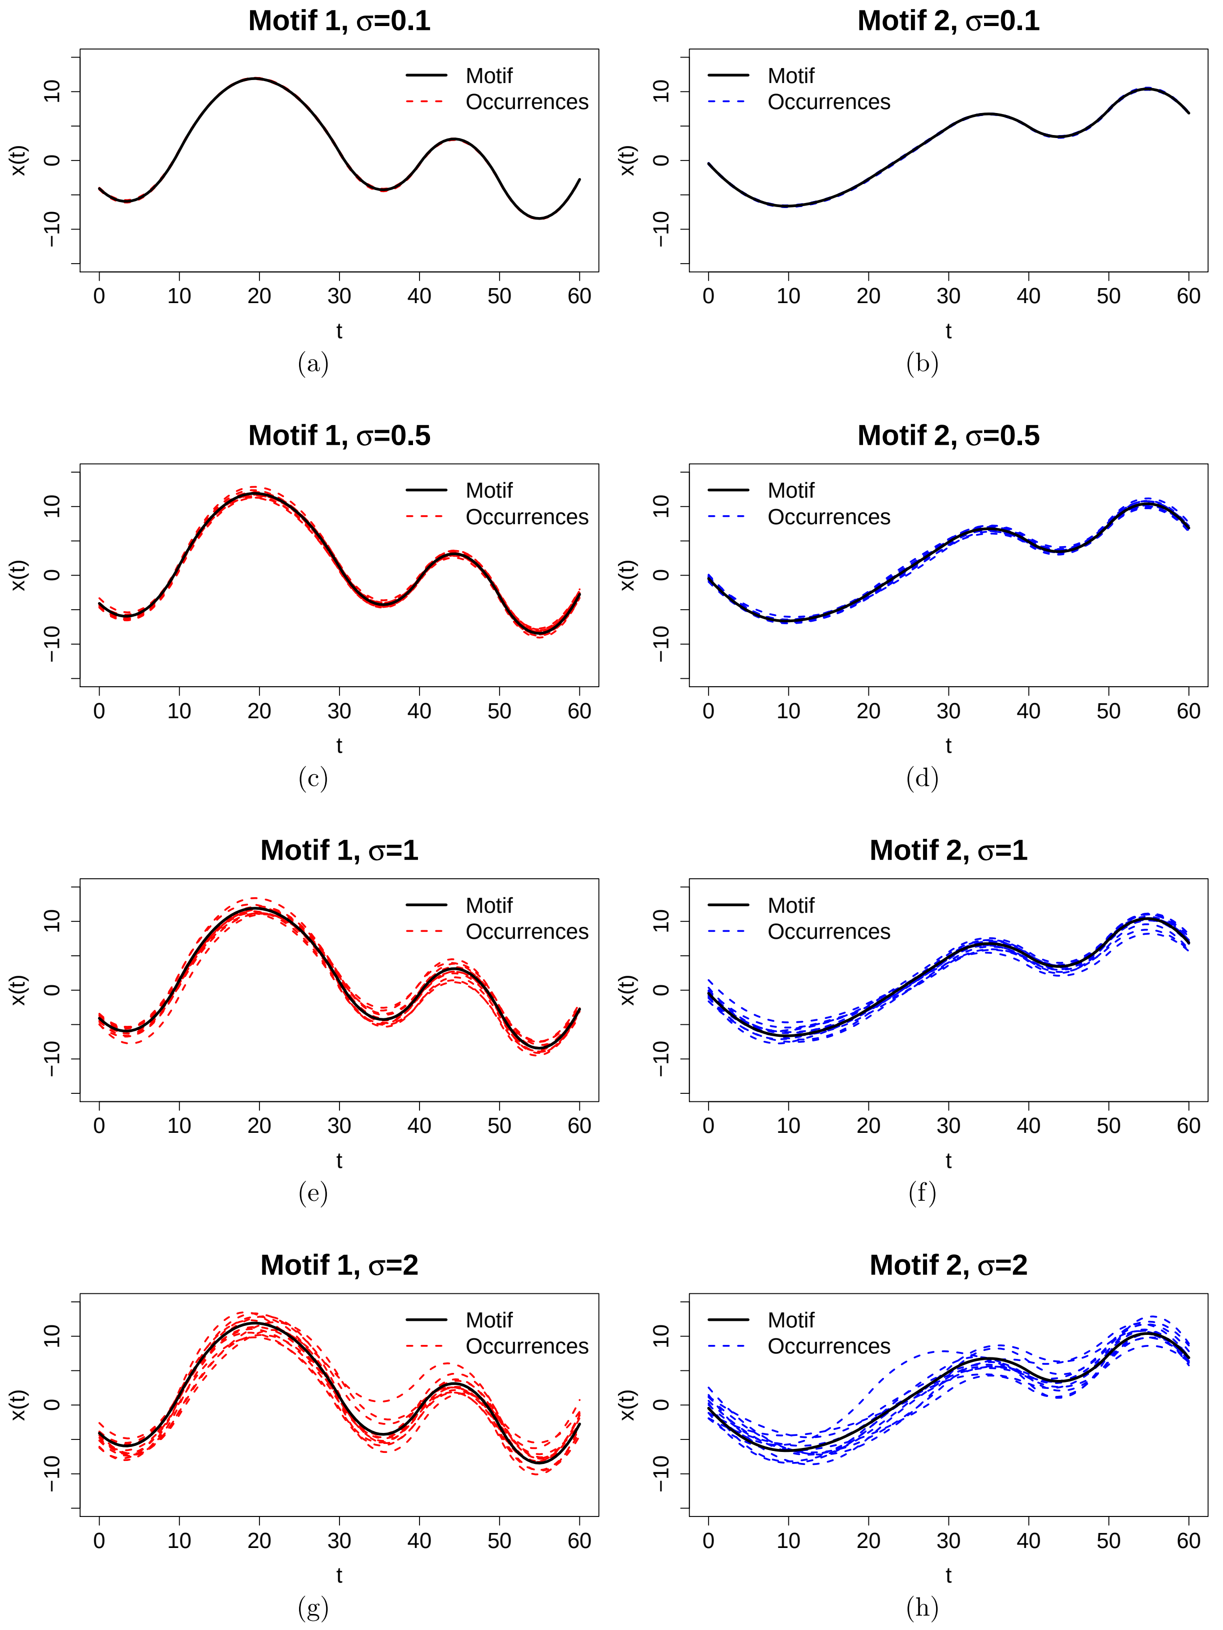


Figure S3: Simulation scenario (1) with $l = 200$. The two functional motifs (black solid lines) and the 12 aligned occurrences of each (red and blue dashed lines) for (a)-(b) $\sigma = 0.1$; (c)-(d) $\sigma = 0.5$; (e)-(f) $\sigma = 1$; (g)-(h) $\sigma = 2$.

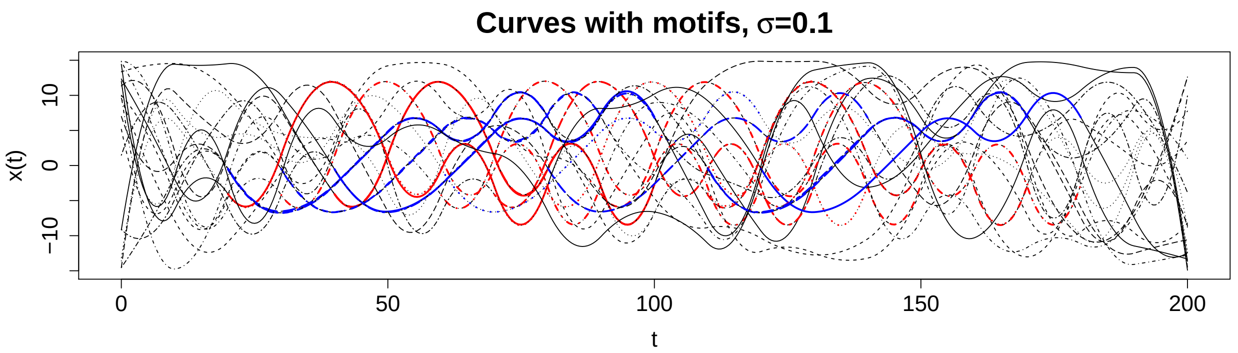


(a)

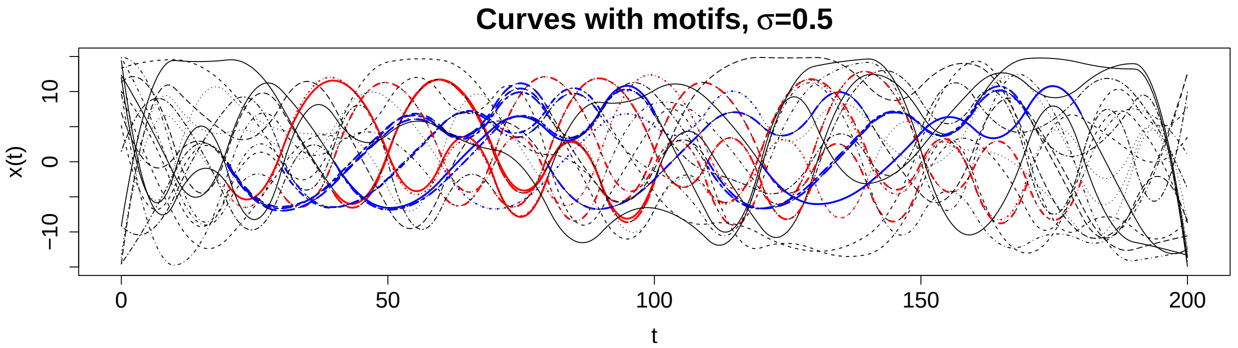


(b)

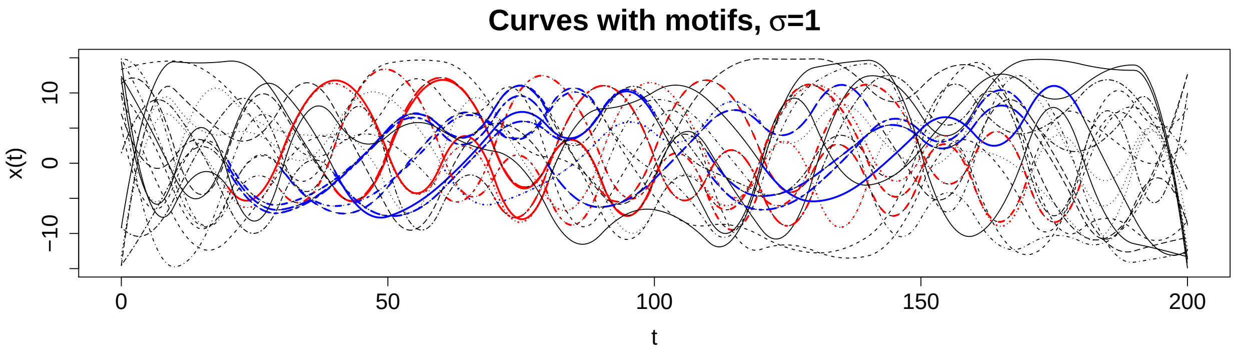


(c)

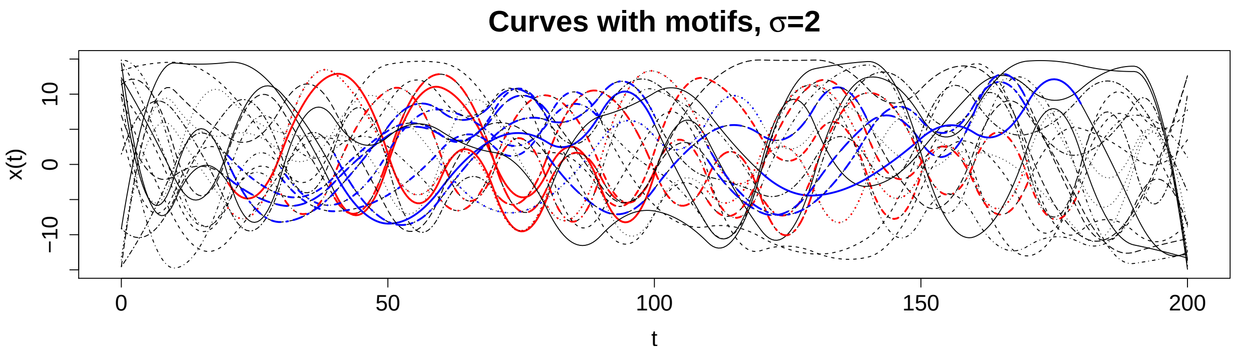


(d)

Figure S4: Simulation scenario (1) with $l = 200$. The 20 curves embedding occurrences of the two motifs (red and blue curve portions, respectively), for (a) $\sigma = 0.1$; (b) $\sigma = 0.5$; (c) $\sigma = 1$; (d) $\sigma = 2$.

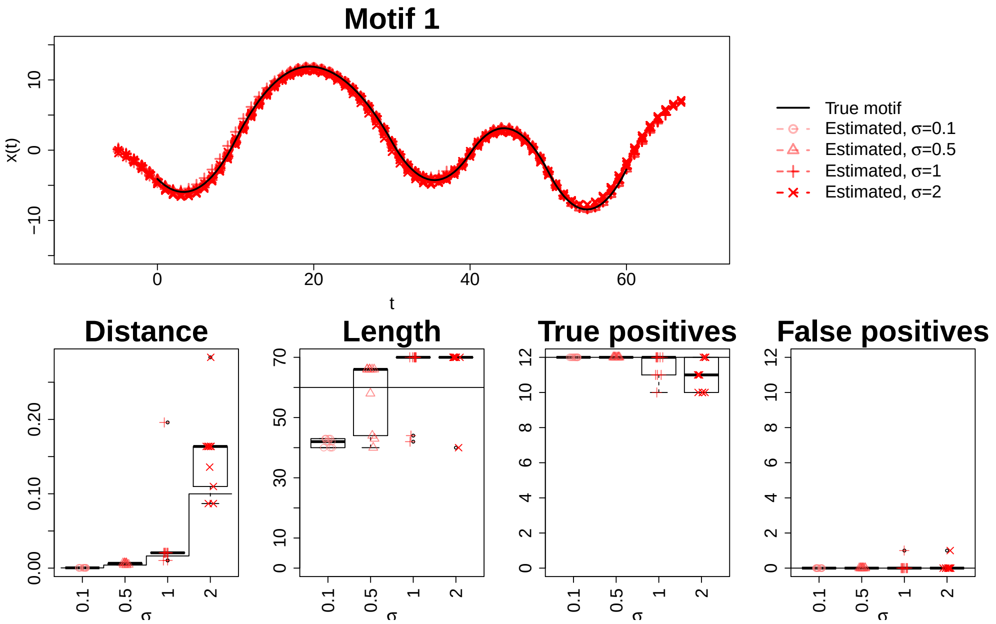


(a)

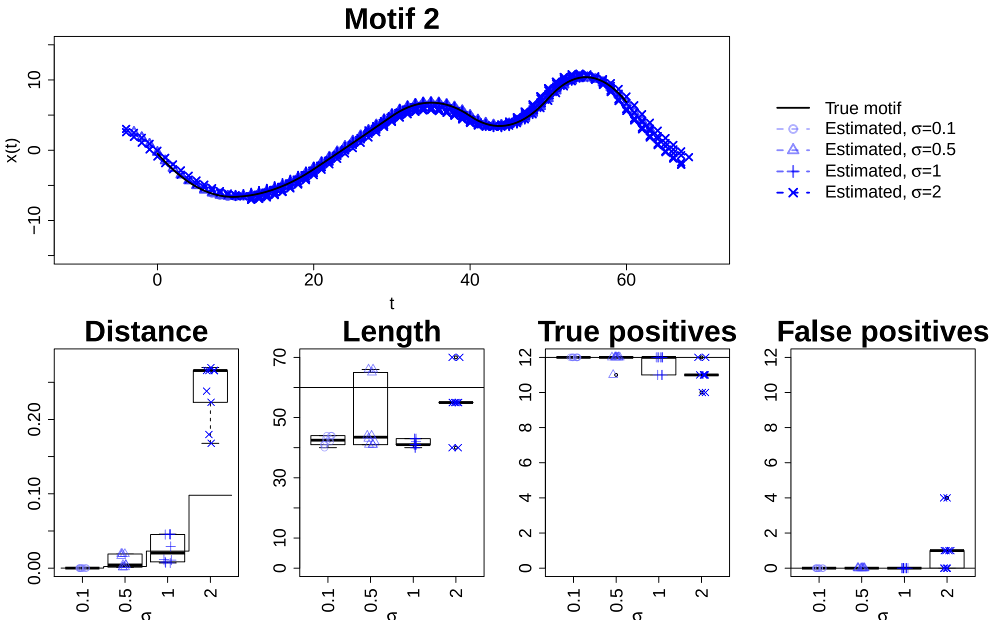


(b)

Figure S5: Functional motif discovery results for simulation scenario (1) with $l = 300$ and various levels of $\sigma$. (a) Motif 1; (b) Motif 2. The boxplots in the lower half of the panels are obtained from 10 replications at each $\sigma$ value. In 33 cases, exactly 2 motifs are found; in the remaining 7 cases, one additional motif is discovered.

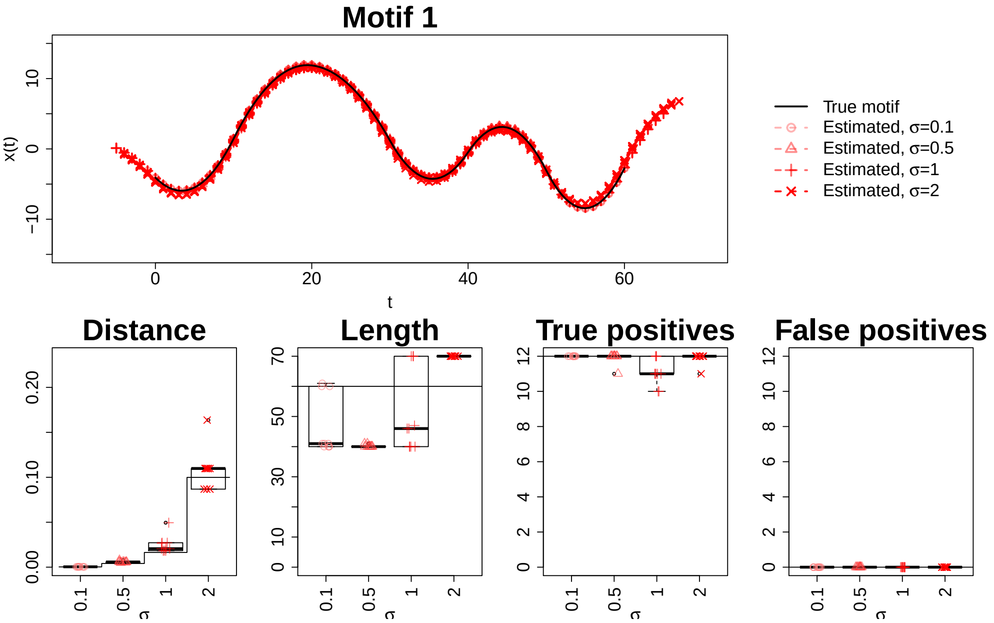


(a)

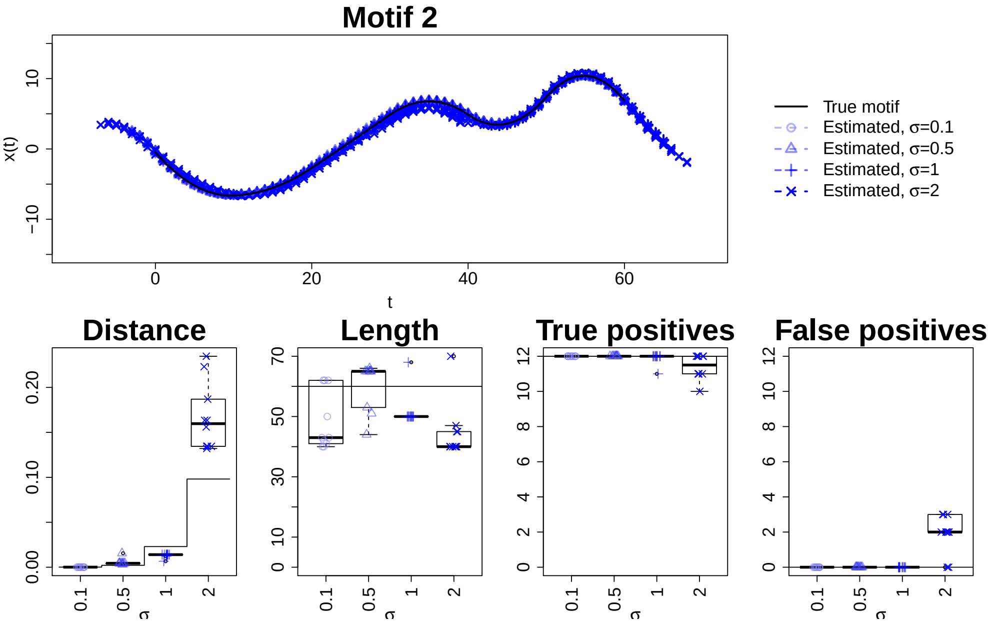


(b)

Figure S6: Functional motif discovery results for simulation scenario (1) with $l = 400$ and various levels of $\sigma$. (a) Motif 1; (b) Motif 2. The boxplots in the lower half of the panels are obtained from 10 replications at each $\sigma$ value. For all the considered noise levels, exactly 2 motifs are found.

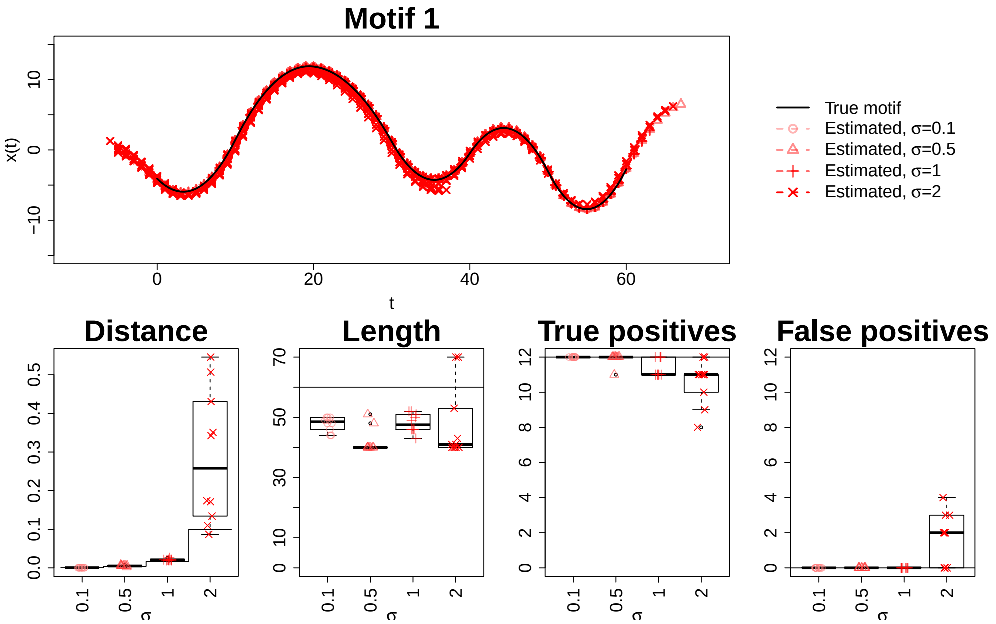


(a)

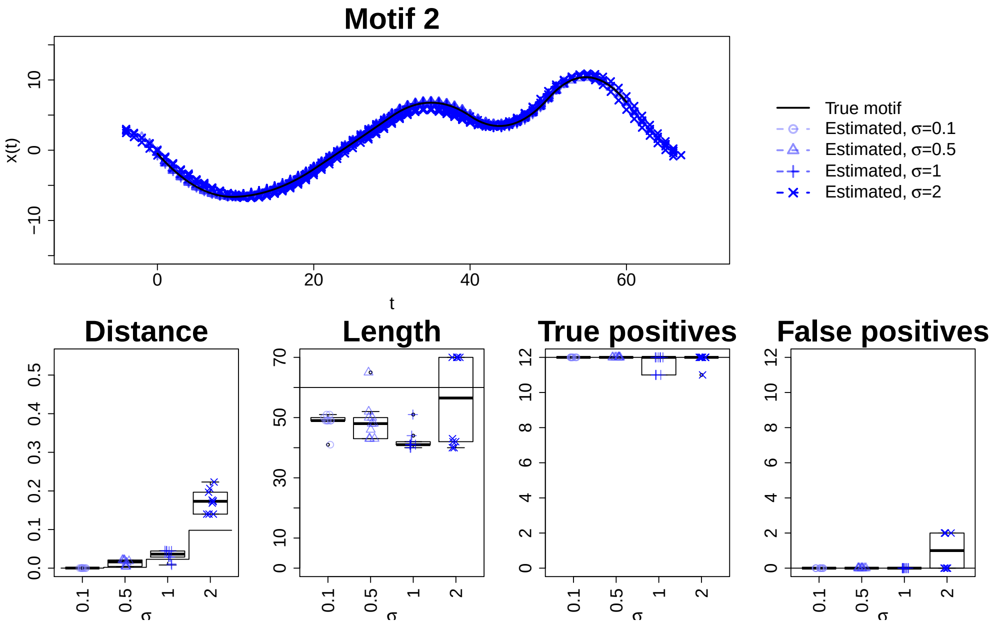


(b)

Figure S7: Functional motif discovery results for simulation scenario (1) with $l = 500$ and various levels of $\sigma$. (a) Motif 1; (b) Motif 2. The boxplots in the lower half of the panels are obtained from 10 replications at each $\sigma$ value. In 34 cases, exactly 2 motifs are found; in the remaining 6 cases, one additional motif is discovered.

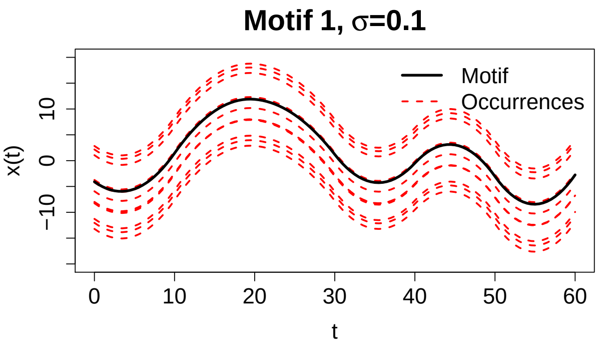

(a)

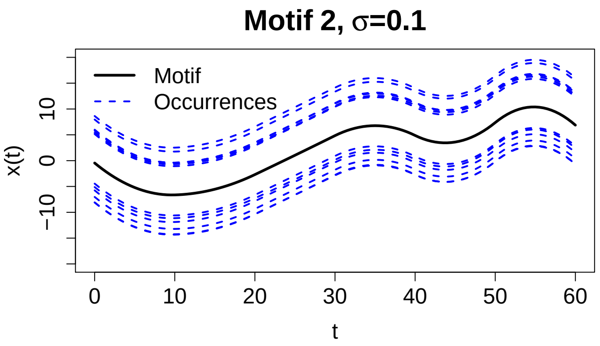

(b)

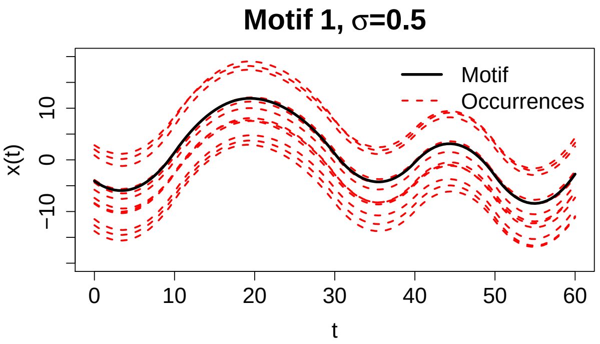

(c)

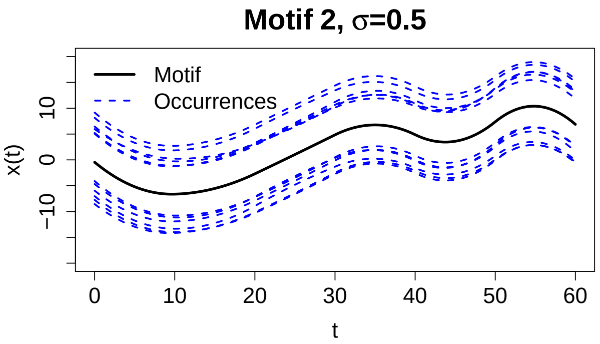

(d)

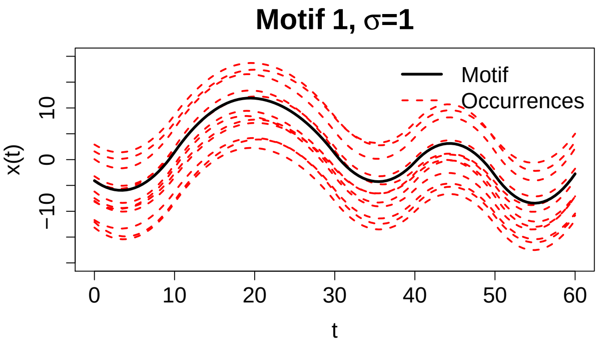

(e)

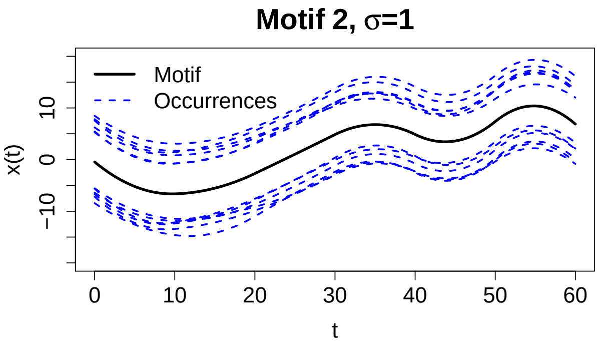

(f)

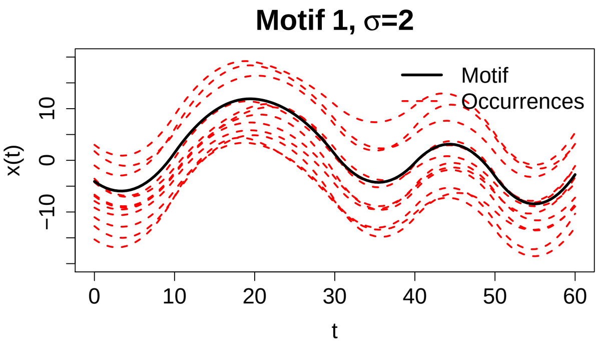

(g)

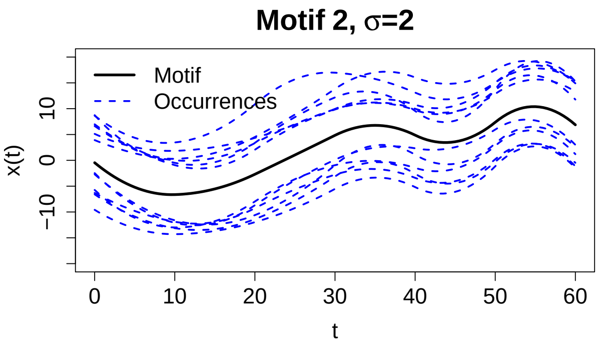

(h)

Figure S8: Simulation scenario (2) with $l = 200$. The two functional motifs (black solid lines) and the 12 aligned occurrences of each (red and blue dashed lines) for (a)-(b) $\sigma = 0.1$; (c)-(d) $\sigma = 0.5$; (e)-(f) $\sigma = 1$; (g)-(h) $\sigma = 2$.

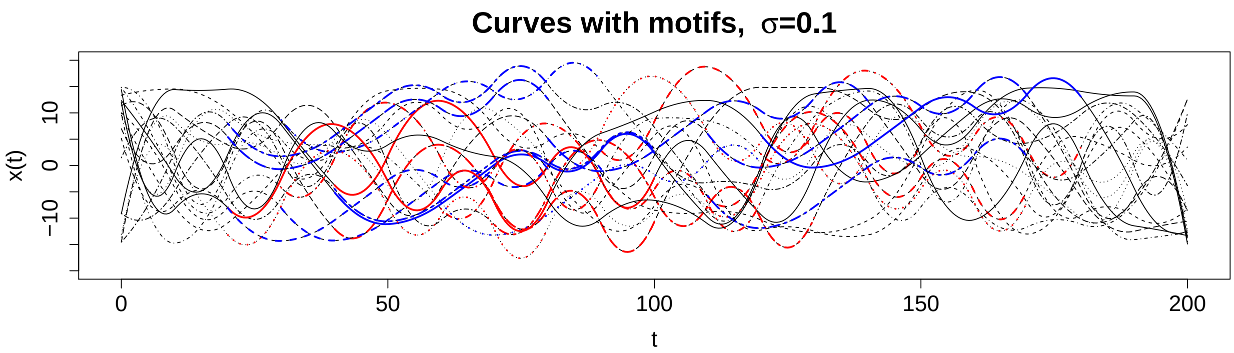


(a)

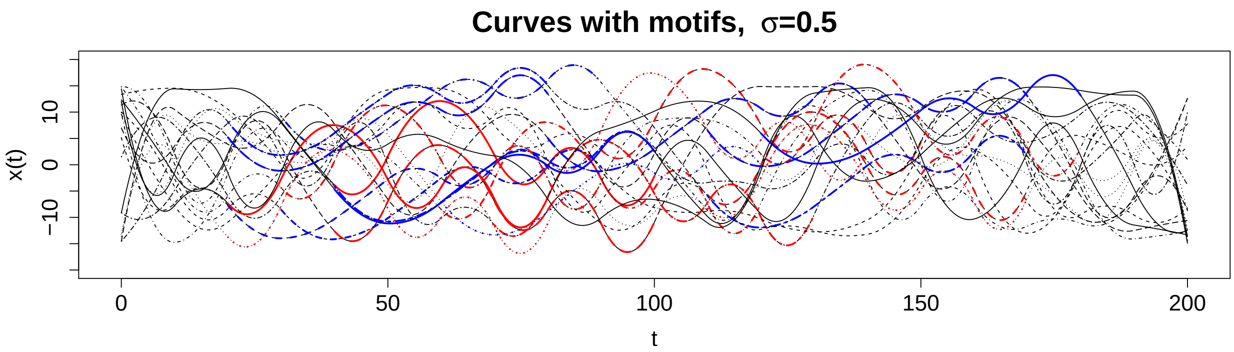


(b)

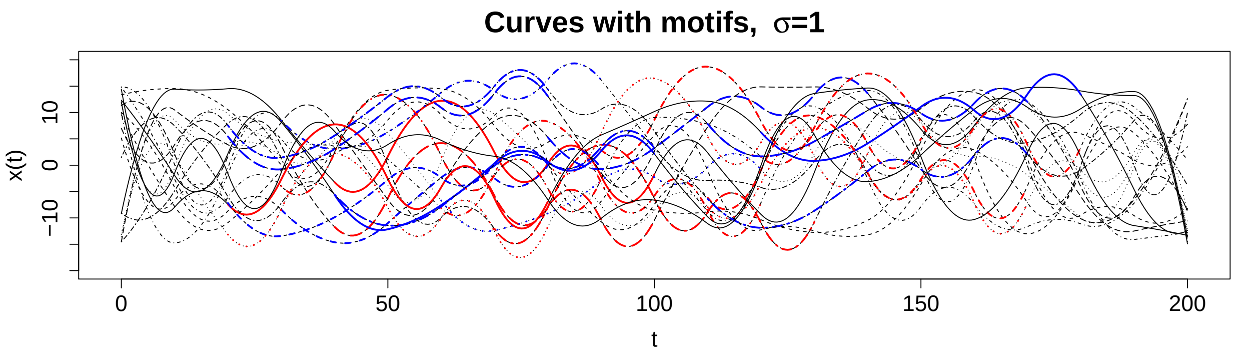


(c)

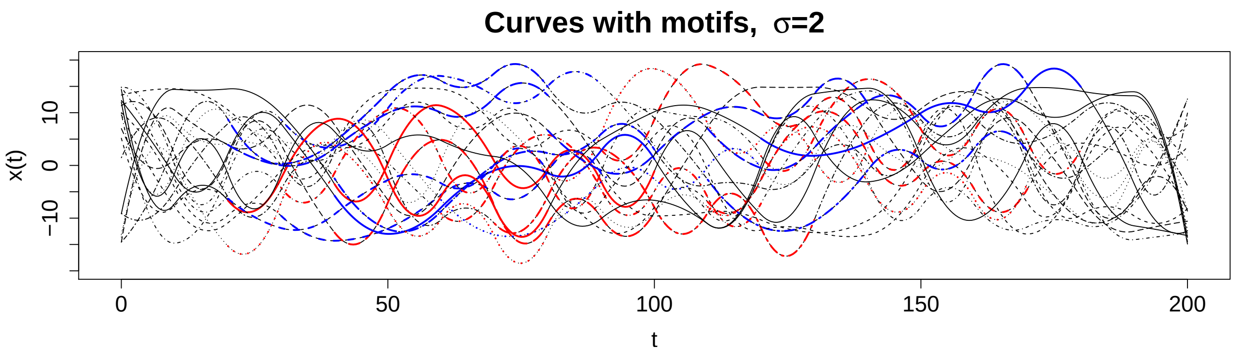


(d)

Figure S9: Simulation scenario (2) with $l = 200$. The 20 curves embedding occurrences of the two motifs (red and blue curve portions, respectively), for (a) $\sigma = 0.1$; (b) $\sigma = 0.5$; (c) $\sigma = 1$; (d) $\sigma = 2$.

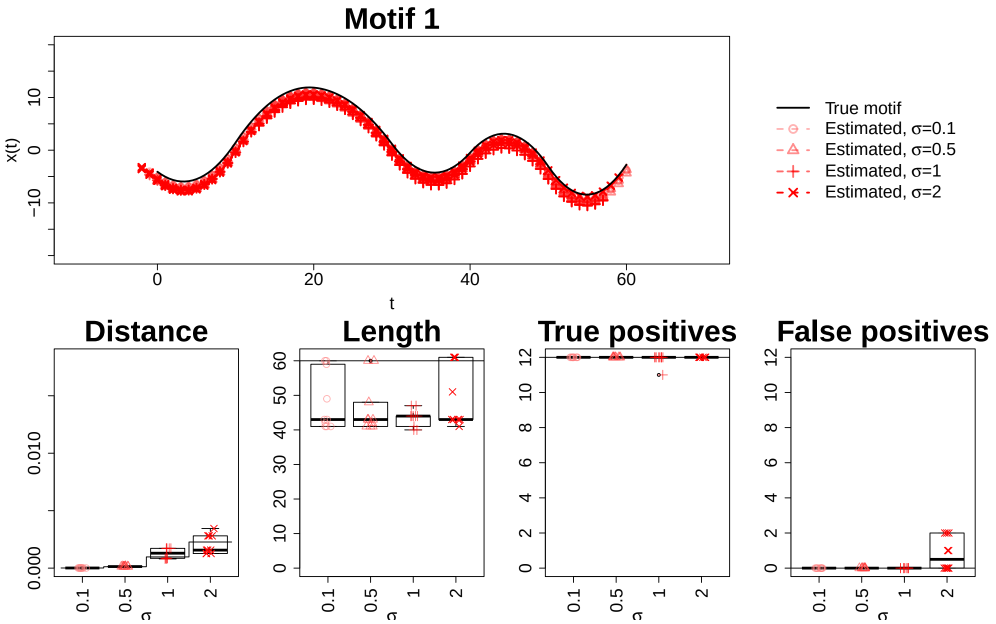


(a)

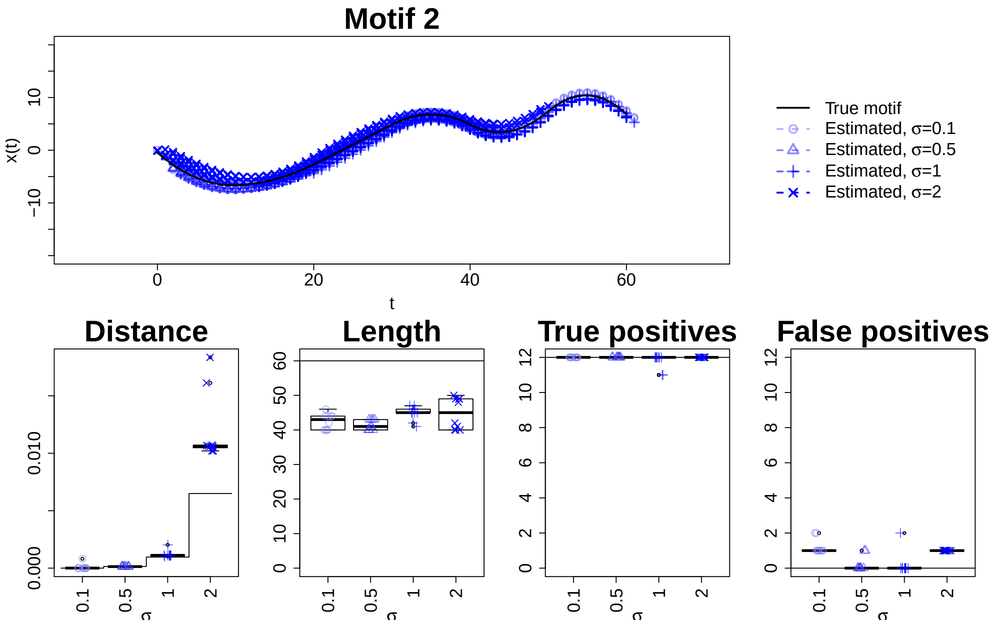


(b)

Figure S10: Functional motif discovery results for simulation scenario (2) with $l = 200$ and various levels of $\sigma$. (a) Motif 1; (b) Motif 2. The boxplots in the lower half of the panels are obtained from 10 replications at each $\sigma$ value. In 34 cases, exactly 2 motifs are found; in 5 cases, one additional motif is discovered; in 1 case, two additional motifs are discovered.

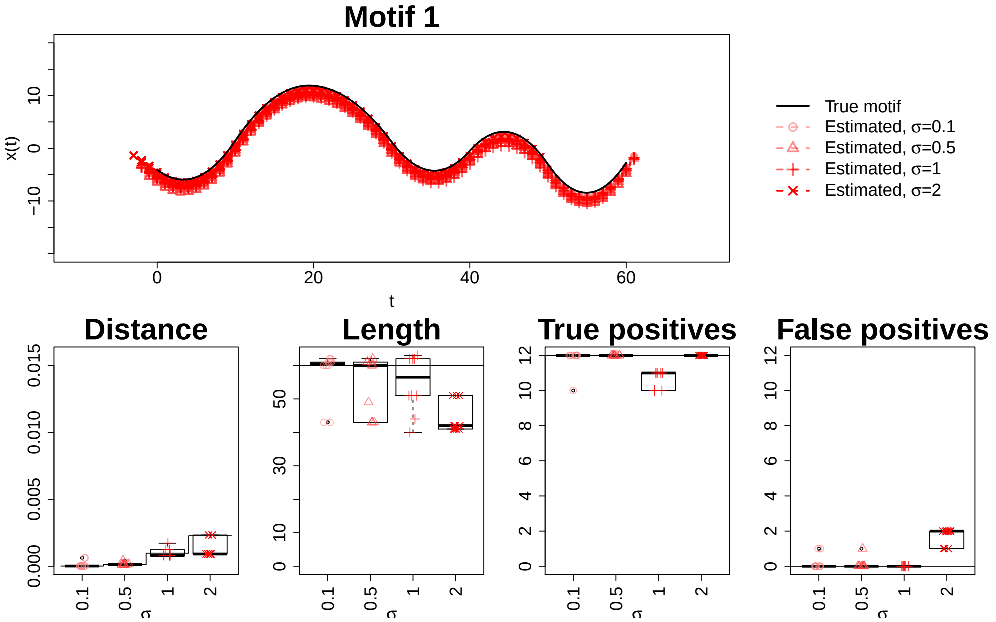


(a)

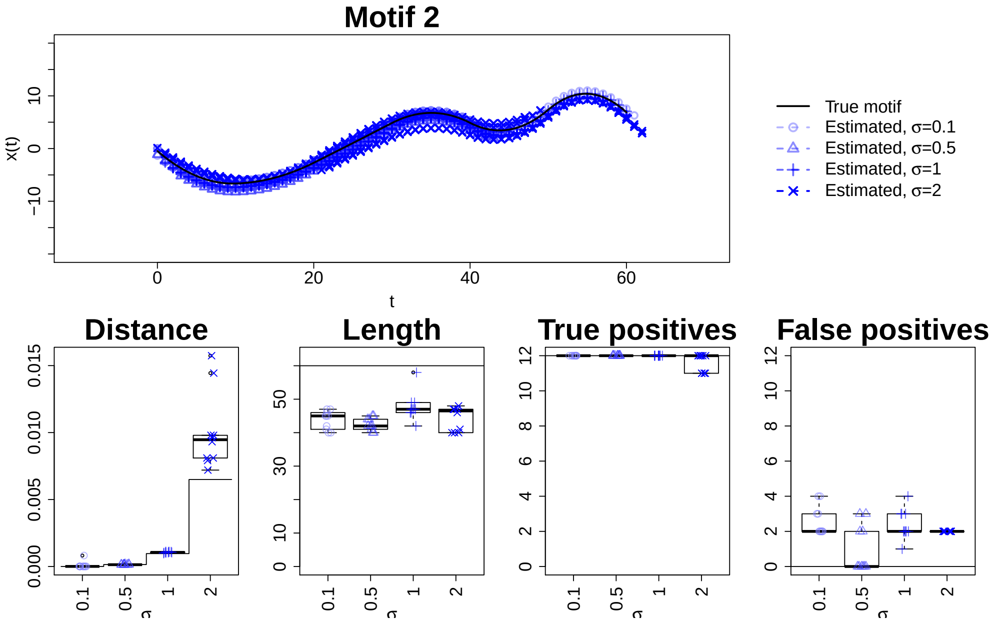


(b)

Figure S11: Functional motif discovery results for simulation scenario (2) with $l = 300$ and various levels of $\sigma$. (a) Motif 1; (b) Motif 2. The boxplots in the lower half of the panels are obtained from 10 replications at each $\sigma$ value. In 16 cases, exactly 2 motifs are found; in 13 cases, one additional motif is discovered; in 11 cases, at least 2 additional motifs are discovered.

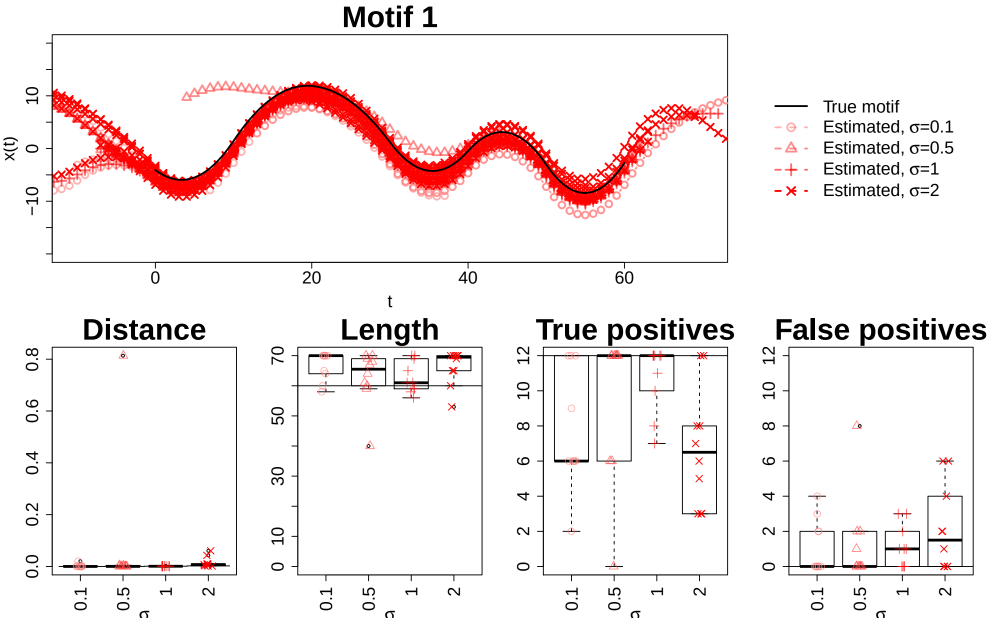


(a)

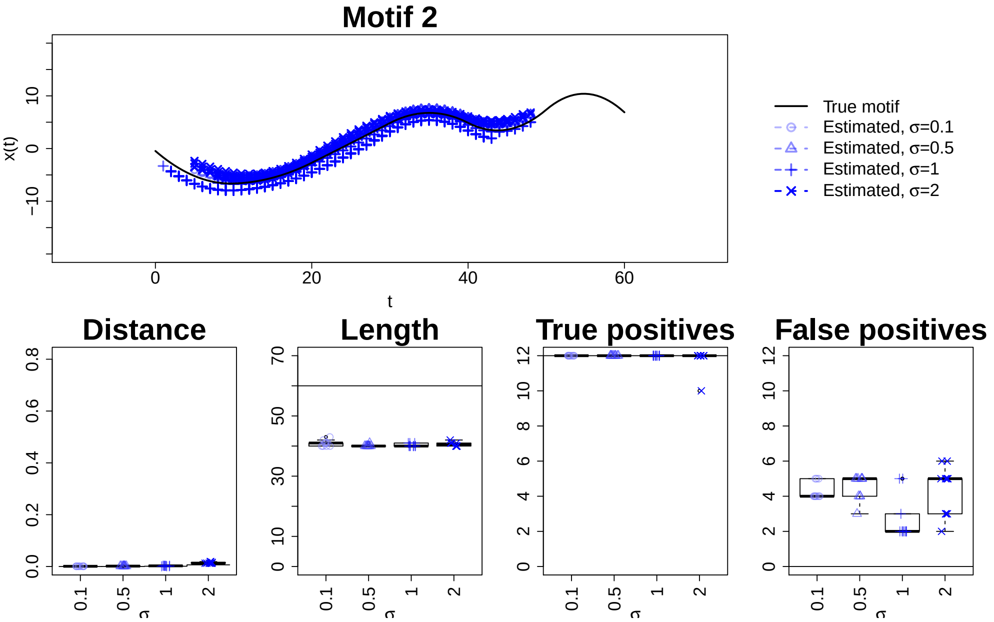


(b)

Figure S12: Functional motif discovery results for simulation scenario (2) with $l = 400$ and various levels of $\sigma$. (a) Motif 1; (b) Motif 2. The boxplots in the lower half of the panels are obtained from 10 replications at each $\sigma$ value. In 2 cases, exactly 2 motifs are found; in 18 cases, one additional motif is discovered; in 20 cases, at least 2 additional motifs are discovered.

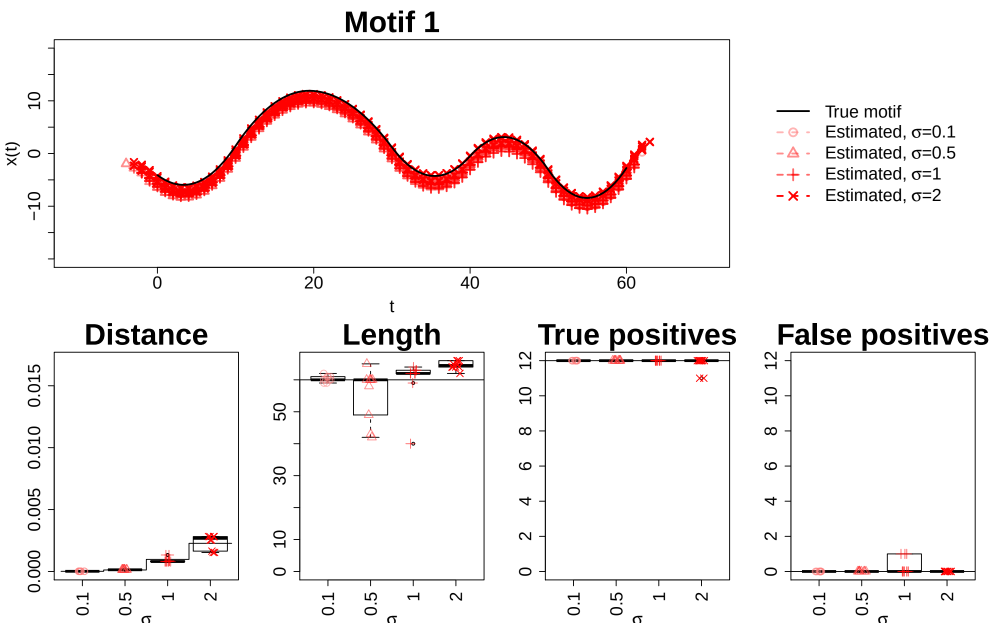


(a)

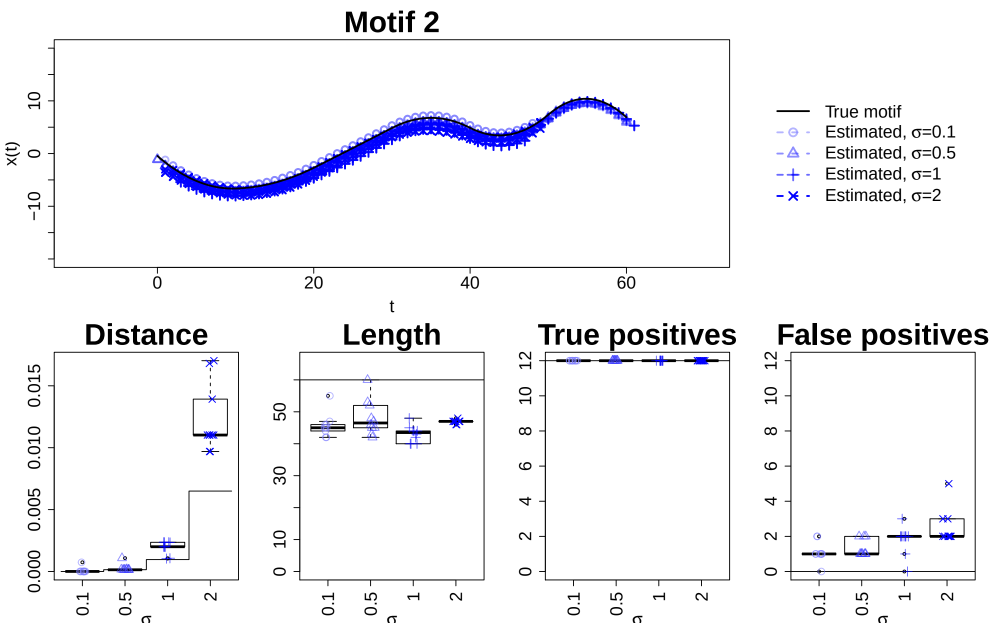


(b)

Figure S13: Functional motif discovery results for simulation scenario (2) with $l = 500$ and various levels of $\sigma$. (a) Motif 1; (b) Motif 2. The boxplots in the lower half of the panels are obtained from 10 replications at each $\sigma$ value. In 16 cases, exactly 2 motifs are found; in 13 cases, one additional motif is discovered; in 25 cases, at least 2 additional motifs are discovered.

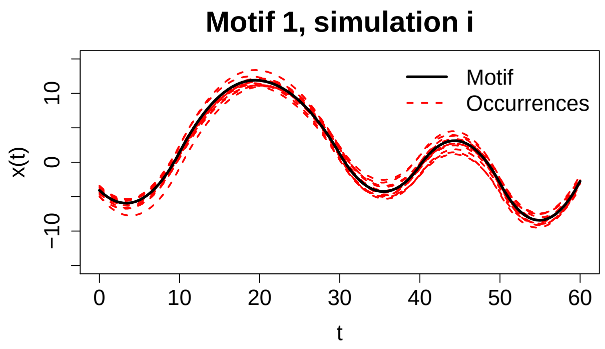
Motif 1, simulation i
Motif
Occurrences
x(t)
−10
0
10
0
10
20
30
40
50
60
t
(a)

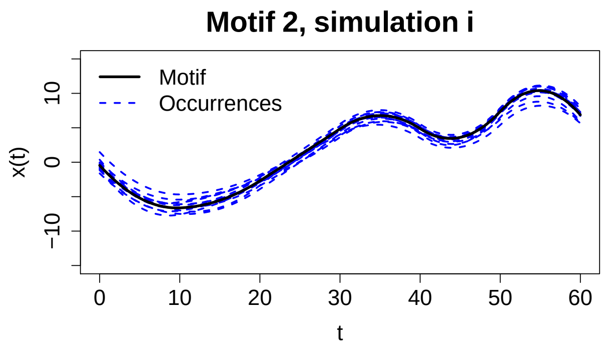
Motif 2, simulation i
Motif
Occurrences
x(t)
−10
0
10
0
10
20
30
40
50
60
t
(b)

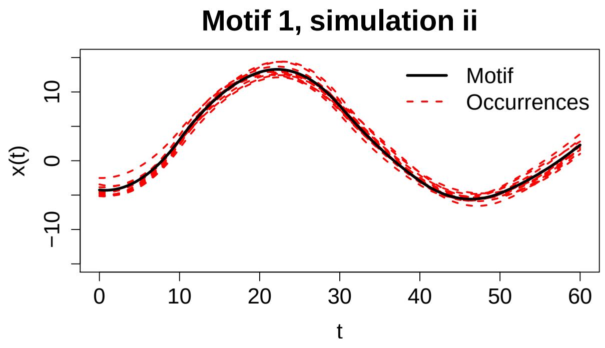
Motif 1, simulation ii
Motif
Occurrences
x(t)
−10
0
10
0
10
20
30
40
50
60
t
(c)

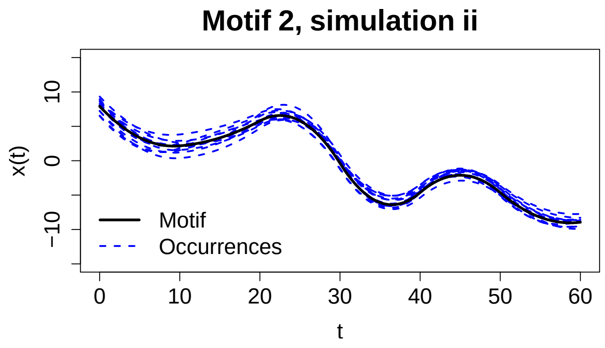
Motif 2, simulation ii
Motif
Occurrences
x(t)
−10
0
10
0
10
20
30
40
50
60
t
(d)

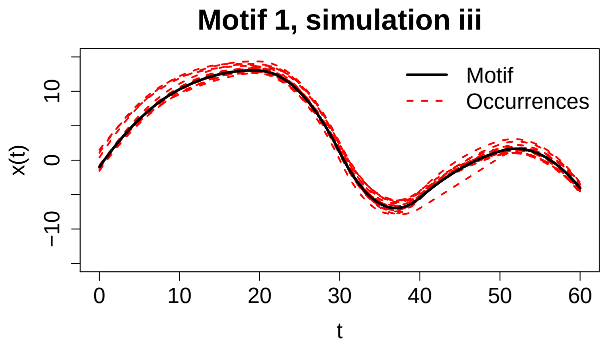
Motif 1, simulation iii
Motif
Occurrences
x(t)
−10
0
10
0
10
20
30
40
50
60
t
(e)

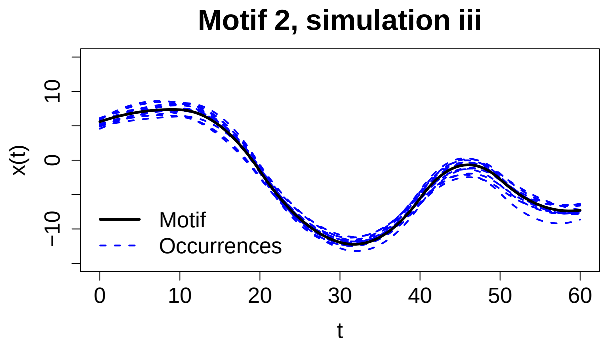
Motif 2, simulation iii
Motif
Occurrences
x(t)
−10
0
10
0
10
20
30
40
50
60
t
(f)

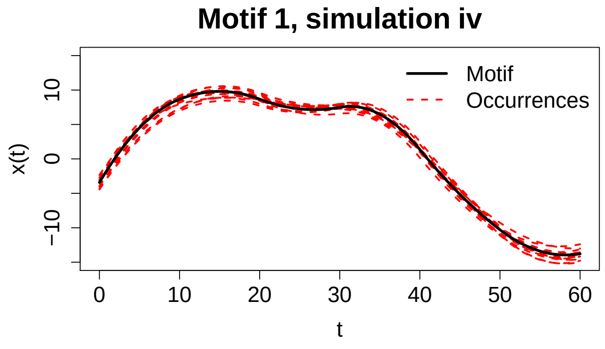
Motif 1, simulation iv
Motif
Occurrences
x(t)
−10
0
10
0
10
20
30
40
50
60
t
(g)

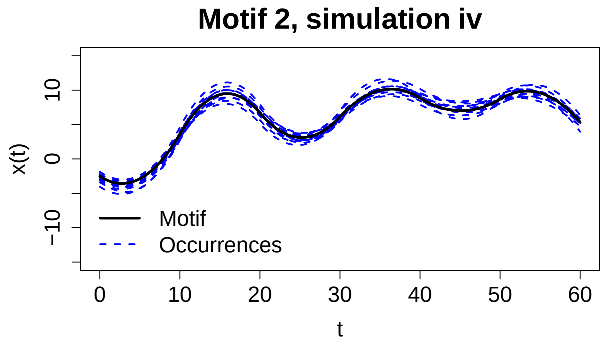
Motif 2, simulation iv
Motif
Occurrences
x(t)
−10
0
10
0
10
20
30
40
50
60
t
(h)

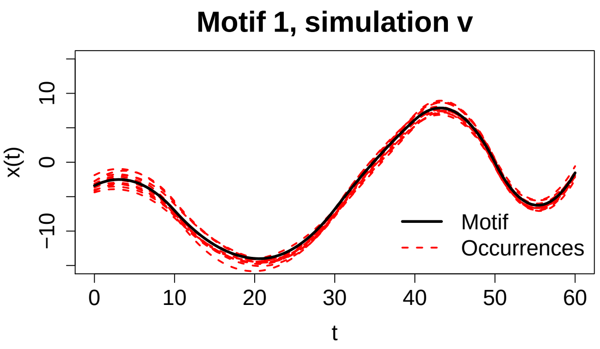
Motif 1, simulation v
x(t)
t
Motif
Occurrences

(i)

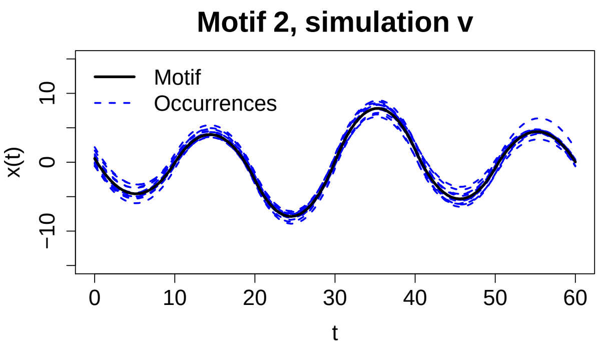
Motif 2, simulation v
x(t)
t
Motif
Occurrences

(j)

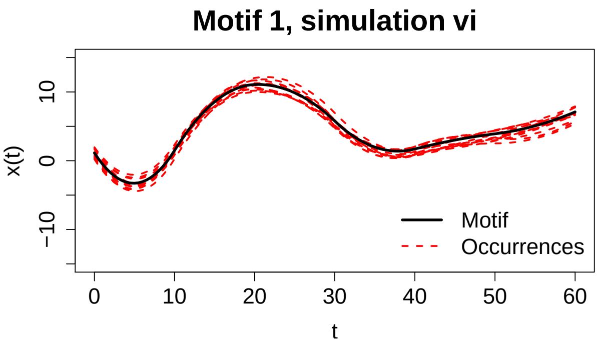
Motif 1, simulation vi
x(t)
t
Motif
Occurrences

(k)

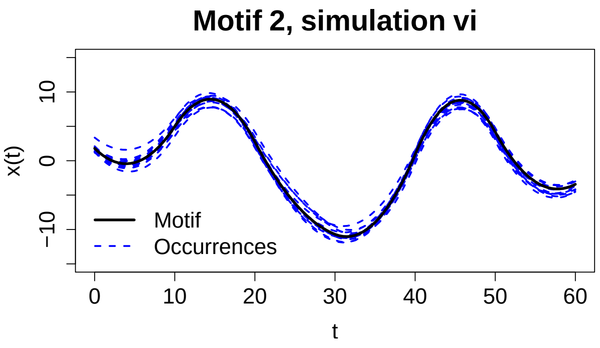
Motif 2, simulation vi
x(t)
t
Motif
Occurrences

(l)

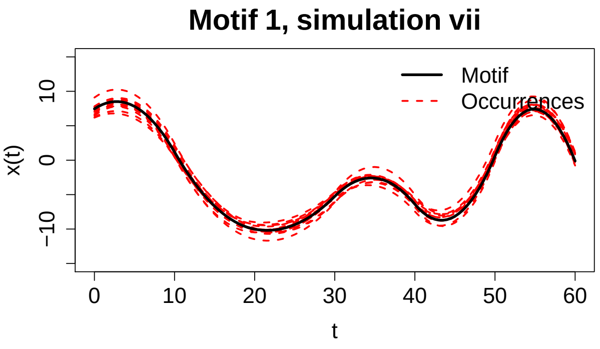
Motif 1, simulation vii
x(t)
t
Motif
Occurrences

(m)

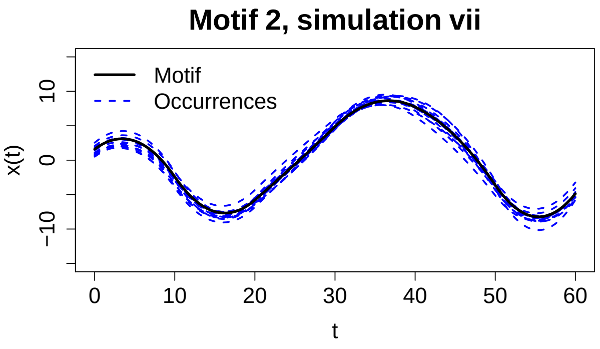
Motif 2, simulation vii
x(t)
t
Motif
Occurrences

(n)

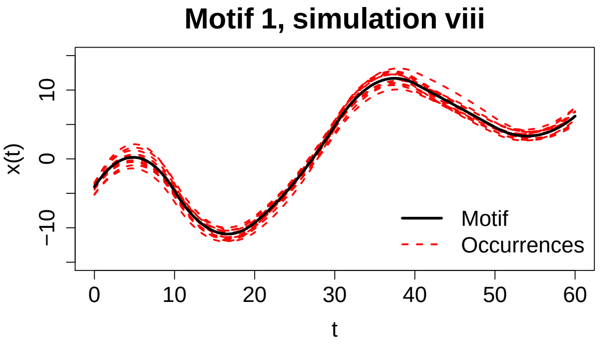
Motif 1, simulation viii
x(t)
t
Motif
Occurrences

(o)

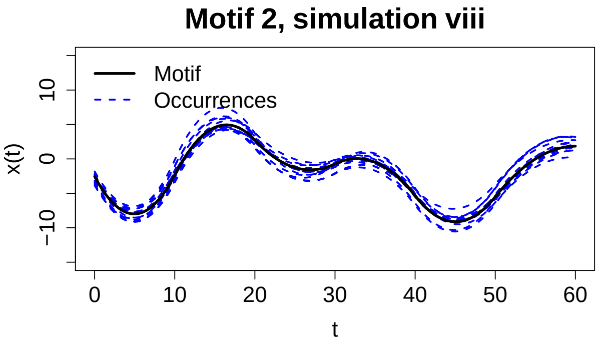
Motif 2, simulation viii
x(t)
t
Motif
Occurrences

(p)

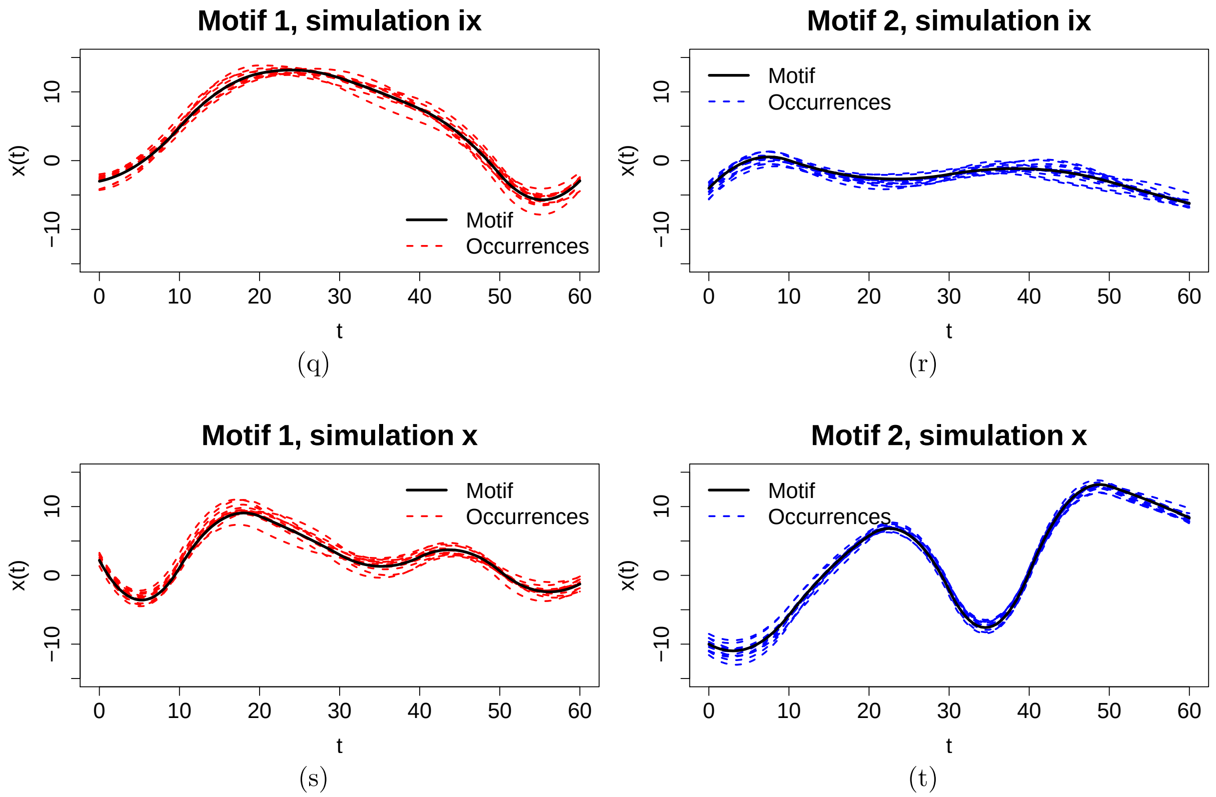


Figure S14: The two functional motifs (black solid lines) and the 12 aligned occurrences of each (red and blue dashed lines), for 10 different datasets in simulation scenario (1), for $l = 200$ and $\sigma = 1$.

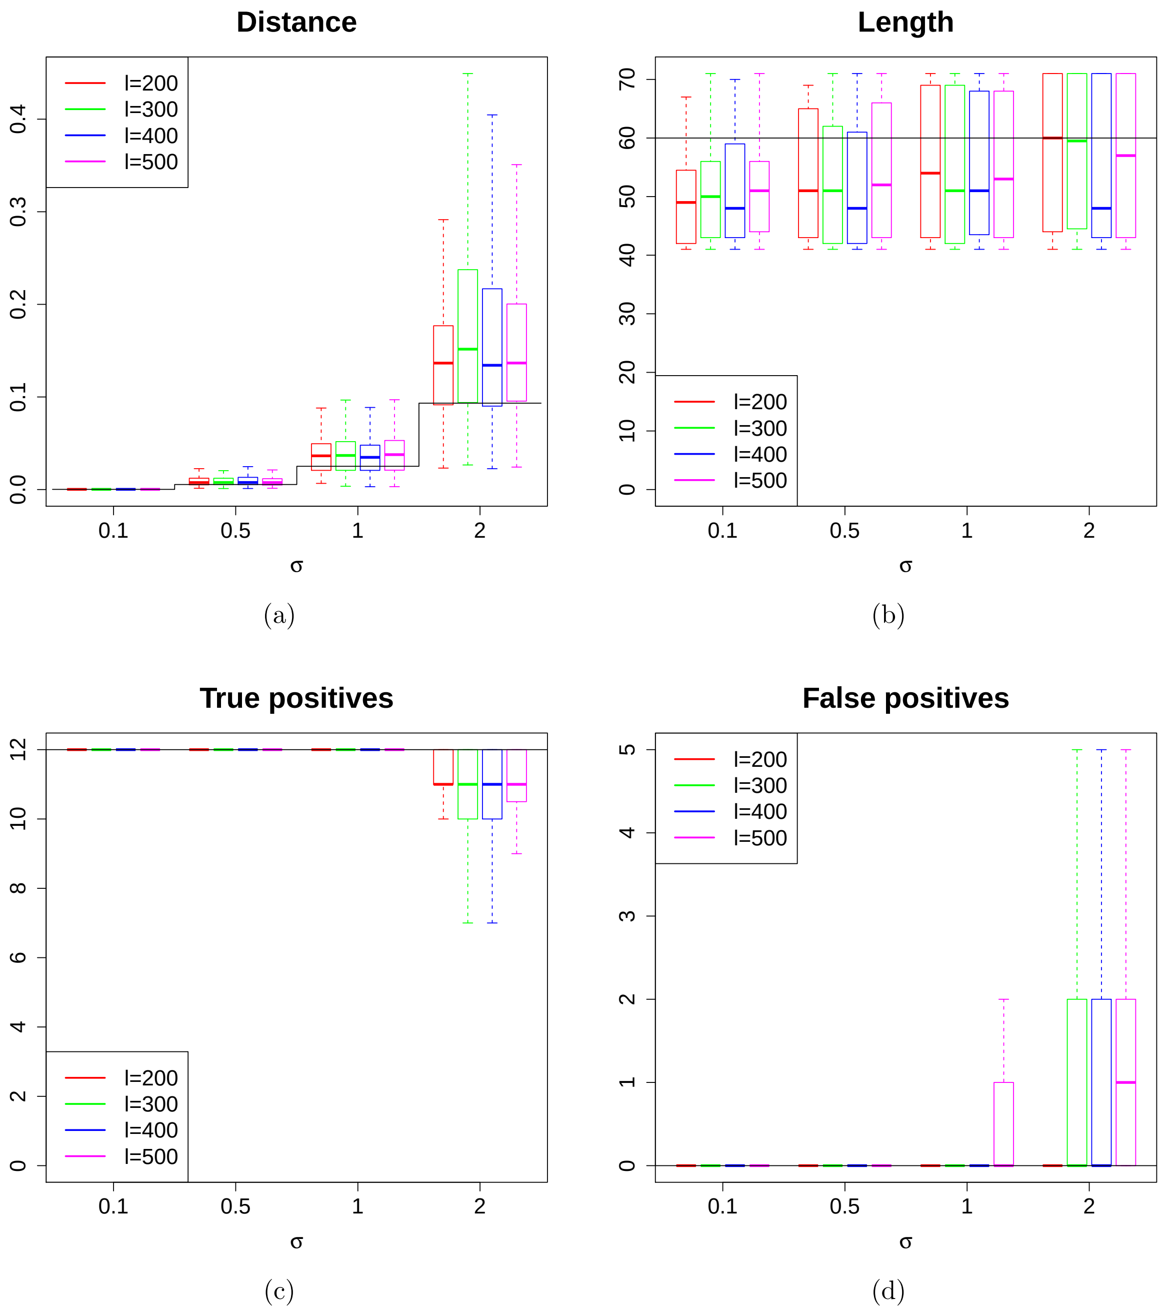


Figure S15: Summary of functional motif discovery results for the 10 different datasets in simulation scenario (1). (a) Distance between true and estimated motifs; (b) Estimated length of motifs; (c) Number of true positives; (d) Number of false positives. The boxplots are obtained from 10 replications at each of the 10 different datasets, and both motifs (a total of 200 observations). Outliers are not plotted, for clarity of visualization.

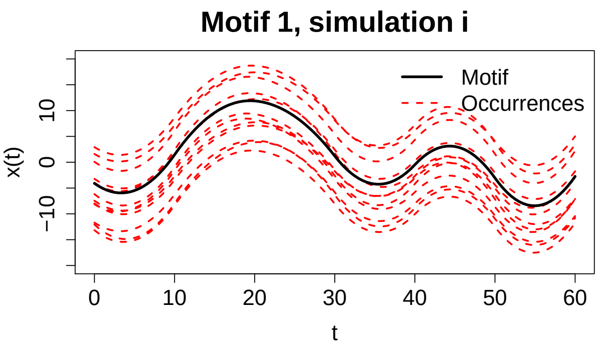
Motif 1, simulation i
Motif
Occurrences
x(t)
t

(a)

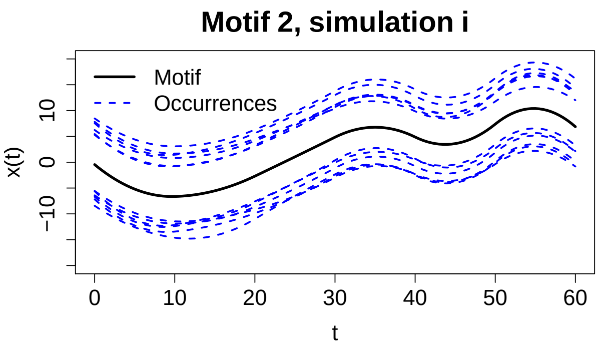
Motif 2, simulation i
Motif
Occurrences
x(t)
t

(b)

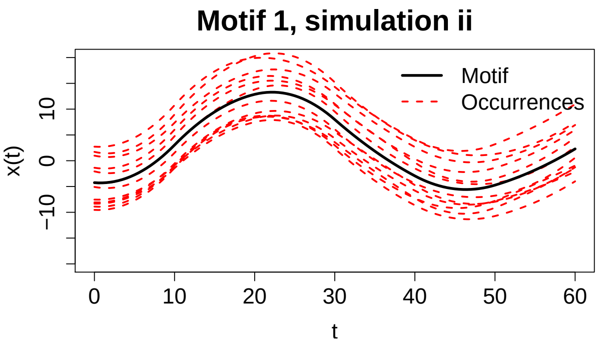
Motif 1, simulation ii
Motif
Occurrences
x(t)
t

(c)

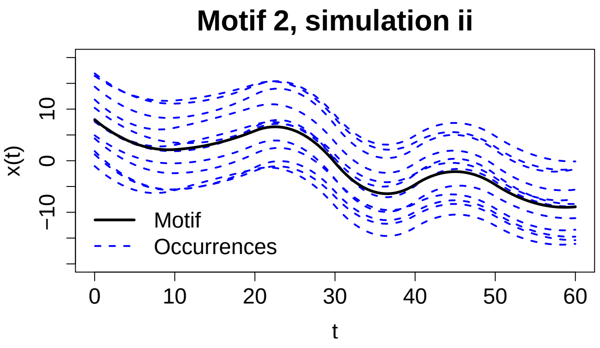
Motif 2, simulation ii
Motif
Occurrences
x(t)
t

(d)

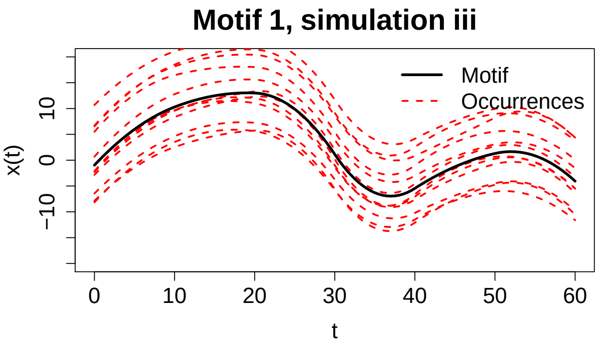
Motif 1, simulation iii
Motif
Occurrences
x(t)
t

(e)

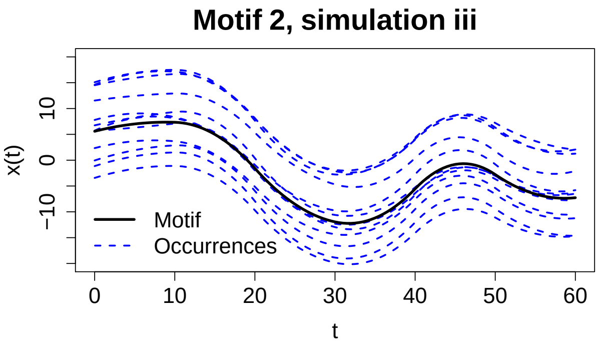
Motif 2, simulation iii
Motif
Occurrences
x(t)
t

(f)

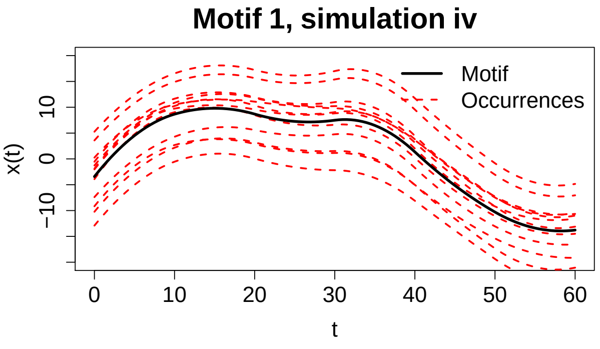
Motif 1, simulation iv
Motif
Occurrences
x(t)
t

(g)

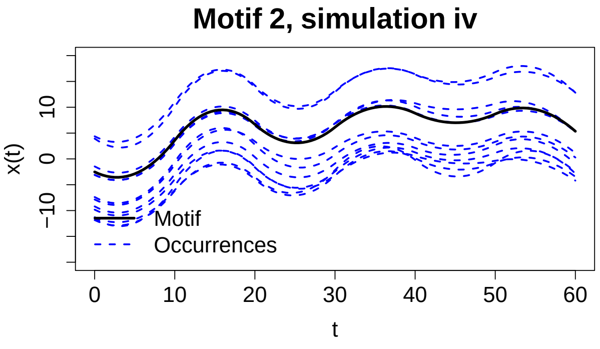
Motif 2, simulation iv
Motif
Occurrences
x(t)
t

(h)

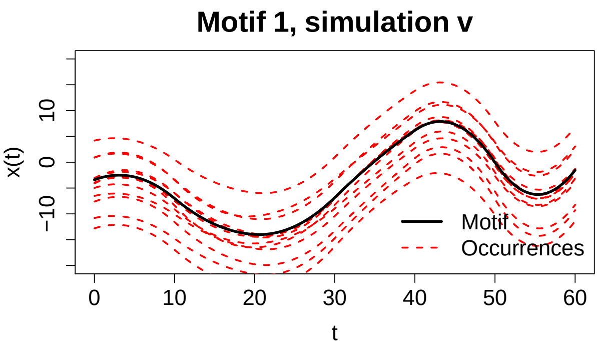
Motif 1, simulation v
x(t)
−10
0
10
0
10
20
30
40
50
60
t
Motif
Occurrences

(i)

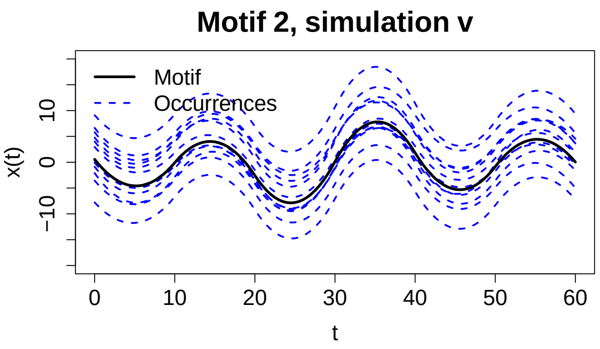
Motif 2, simulation v
x(t)
−10
0
10
0
10
20
30
40
50
60
t
Motif
Occurrences

(j)

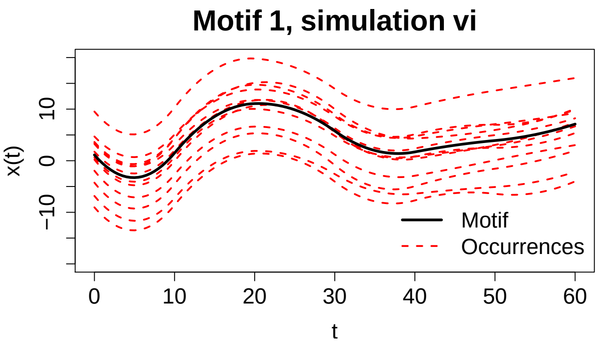
Motif 1, simulation vi
x(t)
−10
0
10
0
10
20
30
40
50
60
t
Motif
Occurrences

(k)

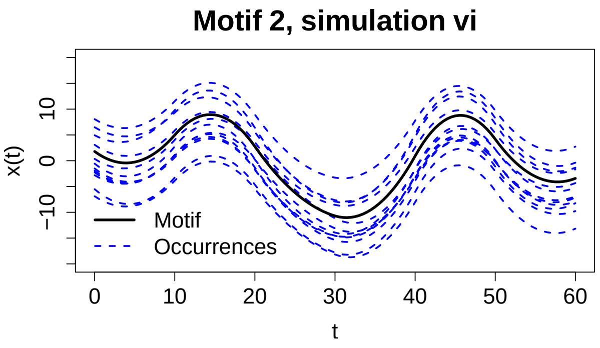
Motif 2, simulation vi
x(t)
−10
0
10
0
10
20
30
40
50
60
t
Motif
Occurrences

(l)

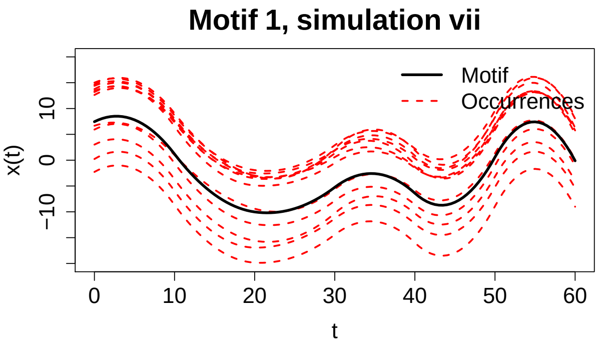
Motif 1, simulation vii
x(t)
−10
0
10
0
10
20
30
40
50
60
t
Motif
Occurrences

(m)

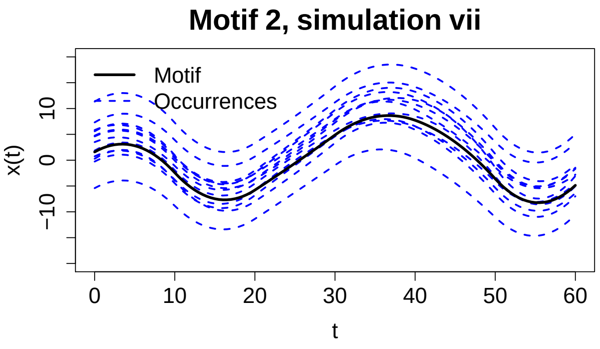
Motif 2, simulation vii
x(t)
−10
0
10
0
10
20
30
40
50
60
t
Motif
Occurrences

(n)

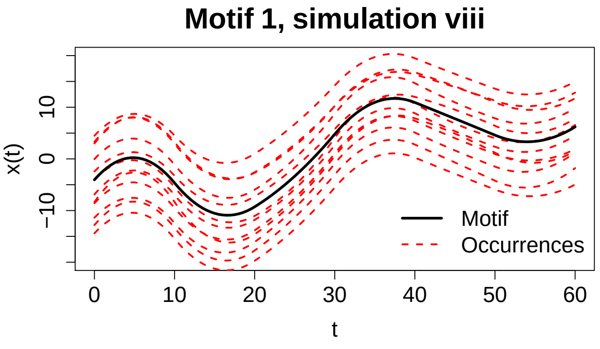
Motif 1, simulation viii
x(t)
−10
0
10
0
10
20
30
40
50
60
t
Motif
Occurrences

(o)

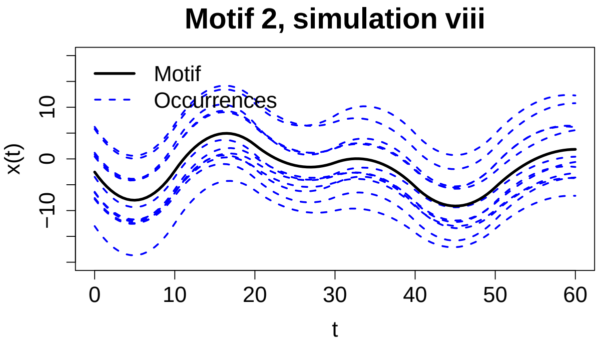
Motif 2, simulation viii
x(t)
−10
0
10
0
10
20
30
40
50
60
t
Motif
Occurrences

(p)

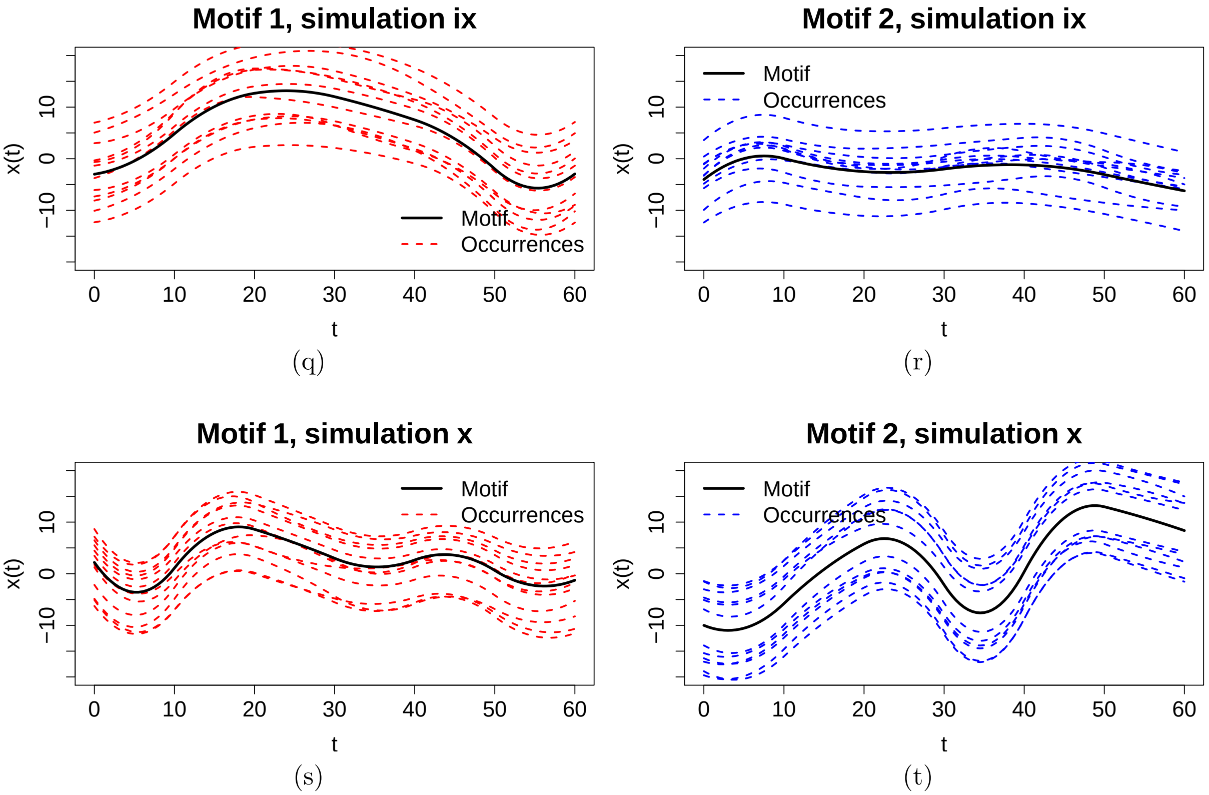


Figure S16: The two functional motifs (black solid lines) and the 12 aligned occurrences of each (red and blue dashed lines), for 10 different datasets in simulation scenario (2), for $l = 200$ and $\sigma = 1$.

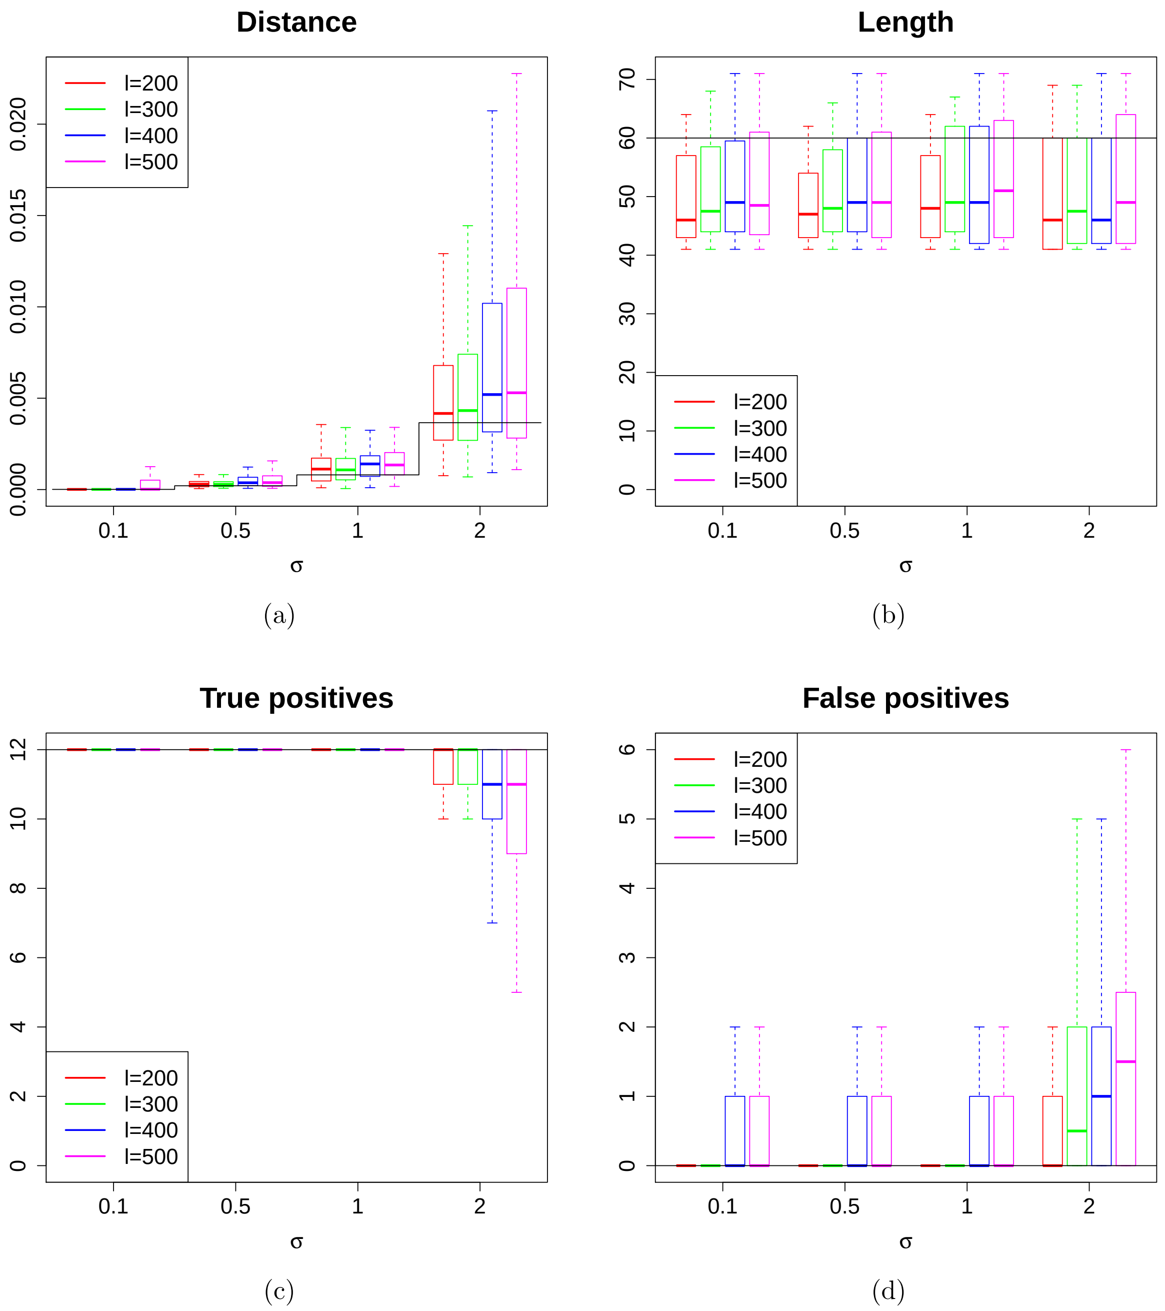


Figure S17: Summary of functional motif discovery results for the 10 different datasets in simulation scenario (2). (a) Distance between true and estimated motifs; (b) Estimated length of motifs; (c) Number of true positives; (d) Number of false positives. The boxplots are obtained from 10 replications at each of the 10 different datasets, and both motifs (a total of 200 observations). Outliers are not plotted, for clarity of visualization.

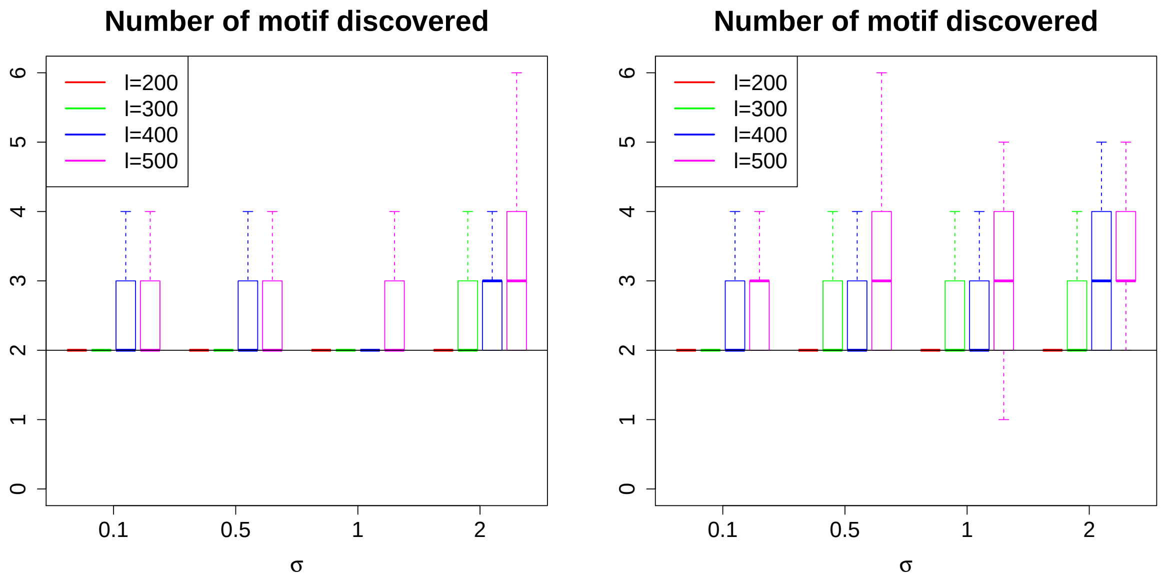


(a) (b)

Figure S18: Number of motifs discovered by functional motif discovery method for the 10 different datasets in (a) simulation scenario (1) and (b) simulation scenario (2). The boxplots are obtained from 10 replications at each of the 10 different datasets (a total of 100 observations). Outliers are not plotted, for clarity of visualization.

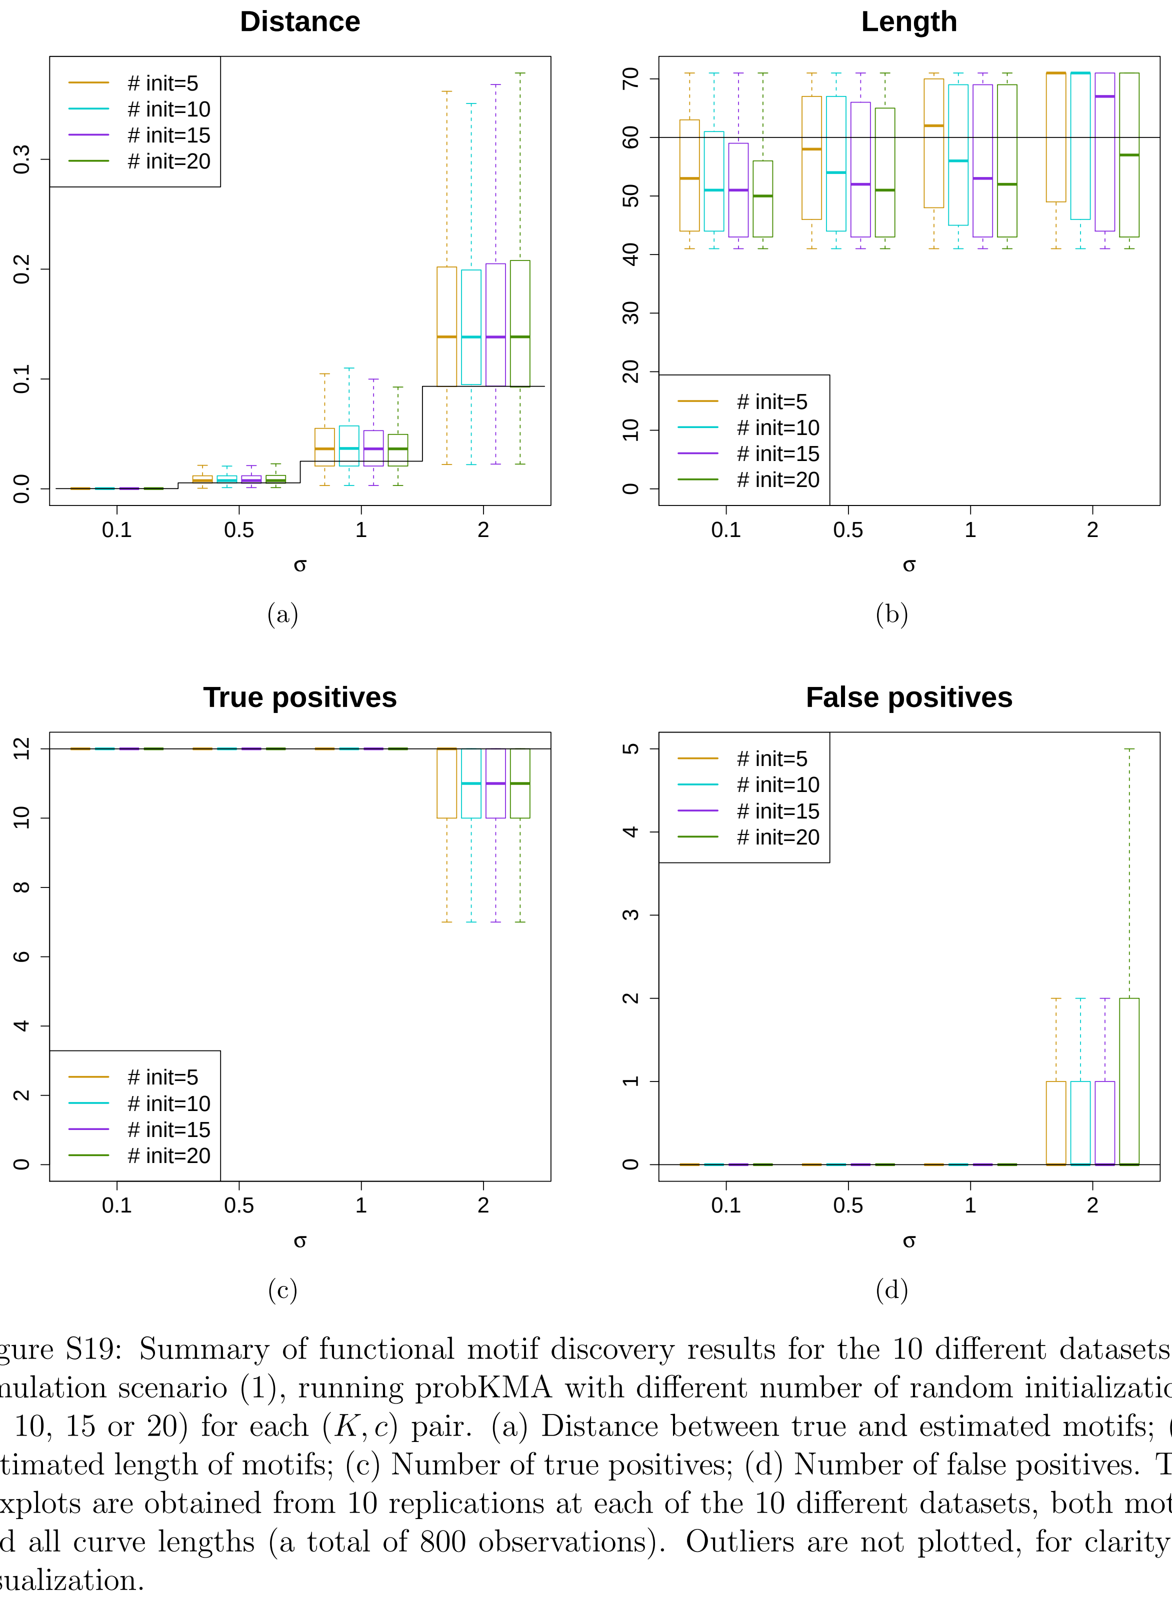


Figure S19: Summary of functional motif discovery results for the 10 different datasets in simulation scenario (1), running probKMA with different number of random initializations (5, 10, 15 or 20) for each $(K, c)$ pair. (a) Distance between true and estimated motifs; (b) Estimated length of motifs; (c) Number of true positives; (d) Number of false positives. The boxplots are obtained from 10 replications at each of the 10 different datasets, both motifs and all curve lengths (a total of 800 observations). Outliers are not plotted, for clarity of visualization.

## S3.2 Comparison to time series motif discovery

Here we report additional information related to the comparison of our probKMA-based functional motif discovery to time series motif discovery (Matrix Profile), discussed in Subsection 4.3.

The *definition of motif* in time series is different from the one we employ for functional data. In particular, given a time series, a motif length $c$, and a radius $R$, Lin et al. (2002) define the most significant motif *1-motif* as the subsequence of length $c$ that has the highest count of matches, i.e. of pieces in the time series with distance less than $R$. Mueen et al. (2009) defines the most basic variant of *1-motif pair* as the most similar pair of pieces of length $c$ in a time series. Yeh et al. (2016, 2018) propose an algorithm, called *Matrix Profile*, to retrieve the nearest neighbor of every subsequence of length $c$. This information is used to select the top motif pairs in the time series. For each motif pair, all neighbors within distance $R$ (i.e. all motif pair matches) can then be retrieved.

We compare our probKMA-based functional motif discovery to *Matrix Profile*, as implemented by the algorithm SCRIMP that is available online at `http://www.cs.ucr.edu/~eamonn/MatrixProfile.html`. We employ a slightly modified version of this code, in which the radius $R$ is provided as input by the user (the original code fixes $R = 1$) and the tool provides as output a maximum of 100 neighbors for each of the top 3 motif pairs found (the original code only provides a maximum of 10 neighbors). The distance employed is the $z$-normalized Euclidean distance, that is defined as the Euclidean distance between standardized subsequence and corresponds to a correlation distance between subsequences: $d(T, Q) = \sqrt{2c\,(1 - \mathrm{cor}(T, Q))}$, with $c$ the length of $T$ and $Q$.

Table S1 shows the results for an additional simulation in scenario (1),using motifs in Fig. S14(s)-(t), while Table S2 reports results of the comparison between probKMA-based functional motif discovery and Matrix Profile, for scenario (2). The results are similar to the ones in Table 1: Matrix Profile works very well in the simple case ($l = 200$, $\sigma = 0.1$), but in the complex case ($l = 500$, $\sigma = 2$) it fails to recognize one motif, while at the same time it includes many false positives; probKMA-based functional motif discovery achieve a good performance in both cases. In addition, we observe how the choice of the radius $R$ is of utmost importance in Matrix Profile: if the radius is too small, not all occurrences are found, while if it is too large many false positives might be included. Importantly, the optimal value for the radius depends not only on motif length and on the level of noise, but also on the shapes of the motifs. Indeed, data employed in Tables 1 and S1 have exactly the same motif length and noise level, but the optimal values of radius in the simple case ($l = 200$, $\sigma = 0.1$) are $R = 30$ and $R = 90$, respectively.

Table S1: Comparison of probKMA-based functional motif discovery and Matrix Profile on an additional simulation in scenario (1) using motifs in Fig. S14(s)-(t) (TP: true positives; FP: false positives). For probKMA, we report median results (and standard deviations) across 10 repeated simulations.

| | | probKMA FMD | Matrix Profile | | | | | | | | | | |
|---|---|---|---|---|---|---|---|---|---|---|---|---|---|
| | Radius | — | 1 | 10 | 20 | 30 | 40 | 50 | 70 | 90 | 110 | 130 | 150 |
| $l = 200, \sigma = 0.1$ (simple case) | | | | | | | | | | | | | |
| Motif 1 | TP | **12 (0)** | 0 | 4 | 6 | 6 | 6 | 6 | 6 | **12** | 12 | 12 | 12 |
| | FP | **0 (0)** | 2 | 0 | 0 | 0 | 0 | 0 | 0 | **0** | 0 | 0 | 0 |
| Motif 2 | TP | **12 (0)** | 2 | 9 | 12 | 12 | 12 | 12 | 12 | **12** | 12 | 12 | 12 |
| | FP | **0 (0)** | 0 | 0 | 0 | 0 | 0 | 0 | 0 | **0** | 0 | 0 | 0 |
| $l = 500, \sigma = 2$ (complex case) | | | | | | | | | | | | | |
| Motif 1 | TP | **12 (1.0)** | 0 | 0 | 0 | 0 | 0 | 0 | 1 | 1 | 1 | 0 | 1 |
| | FP | **0 (1.3)** | 2 | 2 | 4 | 4 | 5 | 8 | 10 | 17 | 22 | 27 | 35 |
| Motif 2 | TP | **10 (1.4)** | 2 | 4 | 7 | 8 | 8 | 12 | 12 | 7 | 7 | 12 | 12 |
| | FP | **1 (1.2)** | 0 | 0 | 1 | 2 | 2 | 5 | 13 | 12 | 13 | 29 | 34 |

Table S2: Comparison of probKMA-based functional motif discovery and Matrix Profile on simulation scenario (2) (TP: true positives; FP: false positives). For probKMA, we report median results (and standard deviations) across 10 repeated simulations.

| | | probKMA FMD | Matrix Profile | | | | | | | | | | |
|---|---|---|---|---|---|---|---|---|---|---|---|---|---|
| | Radius | — | 1 | 10 | 20 | 30 | 40 | 50 | 70 | 90 | 110 | 130 | 150 |
| $l = 200, \sigma = 0.1$ (simple case) | | | | | | | | | | | | | |
| Motif 1 | TP | **12 (0)** | 2 | 6 | 8 | **12** | 12 | 12 | 12 | 12 | 12 | 12 | 12 |
| | FP | **0 (0)** | 0 | 0 | 0 | **0** | 0 | 0 | 0 | 0 | 0 | 0 | 0 |
| Motif 2 | TP | **12 (0)** | 2 | 7 | 11 | **12** | 12 | 12 | 12 | 12 | 12 | 12 | 12 |
| | FP | **1 (0)** | 0 | 0 | 0 | **0** | 0 | 0 | 0 | 0 | 0 | 0 | 0 |
| $l = 500, \sigma = 2$ (complex case) | | | | | | | | | | | | | |
| Motif 1 | TP | **12 (0.4)** | 0 | 0 | 0 | 0 | 0 | 0 | 0 | 0 | 2 | 3 | 6 |
| | FP | **0 (0)** | 2 | 2 | 2 | 4 | 6 | 8 | 16 | 27 | 37 | 53 | 68 |
| Motif 2 | TP | **12 (0)** | 2 | 4 | 8 | 11 | 11 | 11 | 12 | 12 | 12 | 12 | 12 |
| | FP | **2 (1.0)** | 0 | 0 | 0 | 1 | 2 | 7 | 13 | 18 | 25 | 29 | 36 |

## S3.3 Comparison with non-sparse and sparse functional clustering methods

Fig. S20 and Table S3 show data and results of an additional comparison between standard functional $K$-means, KMA, sparse clustering and probKMA, in four scenarios: (a) curves in the two clusters are aligned, and they differ on the entire domain; (b) curves in the two clusters are misaligned, and they differ on the entire domain; (c) curves in the two clusters

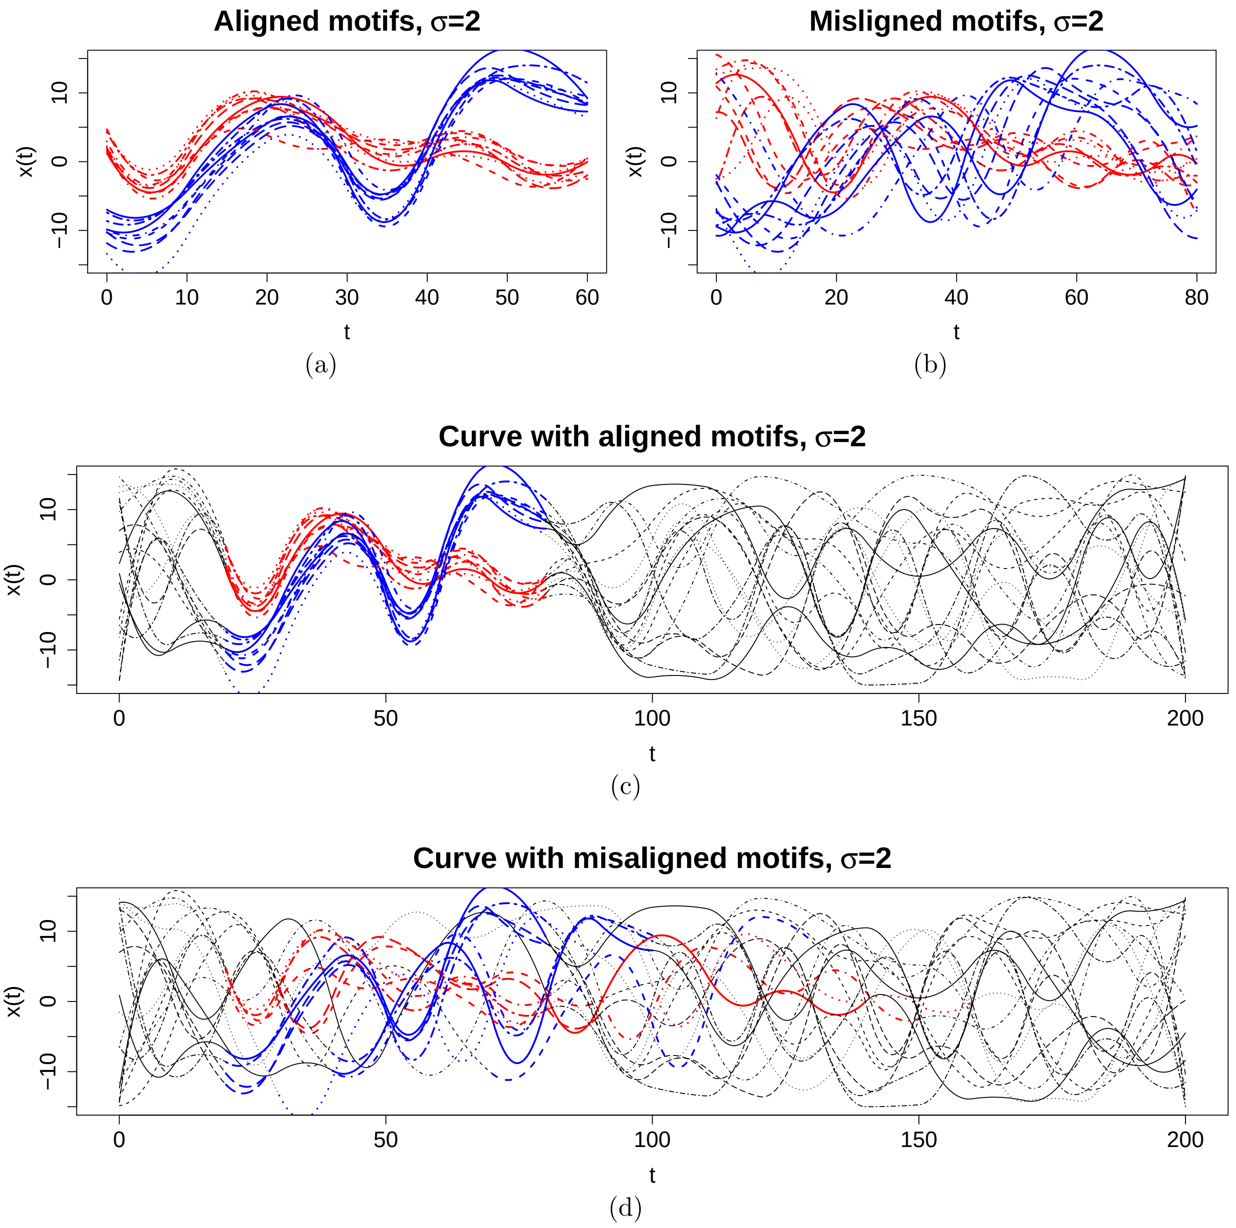


Figure S20: Data for an additional comparison of functional clustering methods, $\sigma = 2$. (a) Aligned motifs; (b) Misaligned motifs; (c) Curves with aligned motifs within them; (d) Curves with misaligned motifs within them. When the curves are broader than the motifs defining the two clusters, the motifs are shown as red and blue lines and the reminder of the curves as black lines.

Table S3: Comparison of probKMA with non-sparse and sparse functional clustering methods in four simulation scenarios. We report means (and standard deviations) of classification error rates across 10 repetitions.

| | Scenario | $K$-means | KMA | sparse | probKMA |
|---|---|---|---|---|---|
| $\sigma = 0.1$ | (a) | **0 (0)** | **0 (0)** | **0 (0)** | **0 (0)** |
| | (b) | 0.11 (0) | 0.08 (0.15) | 0.11 (0) | **0 (0)** |
| | (c) | 0.28 (0.14) | 0.40 (0.19) | 0.14 (0.22) | **0.11 (0.09)** |
| | (d) | 0.48 (0.07) | 0.48 (0.07) | 0.50 (0) | **0.11 (0.10)** |
| $\sigma = 2$ | (a) | **0 (0)** | **0 (0)** | **0 (0)** | **0 (0)** |
| | (b) | 0.11 (0) | 0.12 (0.21) | 0.11 (0) | **0 (0)** |
| | (c) | 0.43 (0.10) | 0.35 (0.15) | 0.19 (0.24) | **0.14 (0.13)** |
| | (d) | 0.46 (0.08) | 0.42 (0.09) | 0.46 (0.05) | **0.09 (0.10)** |

differ on a portion of the domain, and this portion is aligned; (d) curves in the two clusters differ on a portion of the domain, and this portion is misaligned.

# S4 Application to mutagenesis: additional figures and results

We estimate high-resolution neutral mutation rates using the same pipeline as in Kuruppumullage Don et al. (2013). First, we identify neutral DNA by considering all repeats ancestral to human and macaque (AR subgenome, see e.g. Hardison et al., 2003). In particular, we consider the human reference genome hg19 and we select all the repeats (interspersed repeats and low complexity DNA sequences) from RepeatMasker track (Smit et al., 2010) using Galaxy (Blankenberg et al., 2010; Goecks et al., 2010) and excluding L1PA1-7, L1HS, AluY (primate or human specific elements) and Conserved Non-Exonic Elements (CNEEs, putative regulatory regions detected by Lowe and Haussler, 2012). In total, we obtain 5 407 927 AR regions, covering $\sim$ 43% of the entire genome. We then consider the 47 hot regions identified by Kuruppumullage Don et al. (2013). Since these regions are provided on the hg18 release of the human reference genome, we use the lift-over tool (Blankenberg et al., 2010) to convert them to hg19. Requiring that a minimum of 90% of the nucleotides remap to the hg19 release, we are able to retain 43 regions – corresponding to 91.5% of the initial regions. We partition these 43 regions in 1-kb windows, and we discard the ones with less than 25% AR coverage to avoid very inaccurate rate estimates. Afterwards, we extract multiple alignments corresponding to AR subgenome in each 1-kb window, using the 46-way multiZ alignment available in Galaxy (Blankenberg et al., 2011) as depicted in Fig. S21. To estimate substitution rates we fetch pairwise alignments of human and orangutan (ponAbe2 assembly) and we mask low quality nucleotides within each block, requiring an orangutan PHRED score greater than 20. Next, we identify nucleotide substitutions and we estimate the substitution rate in each window as the number of substitutions (i.e. the number of different nucleotides in human and orangutan alignment) divided by the total number of compared nucleotides in the window, using the Jukes-Cantor model (Jukes and Cantor, 1969). Although we require that at least the 25% of each considered window is covered

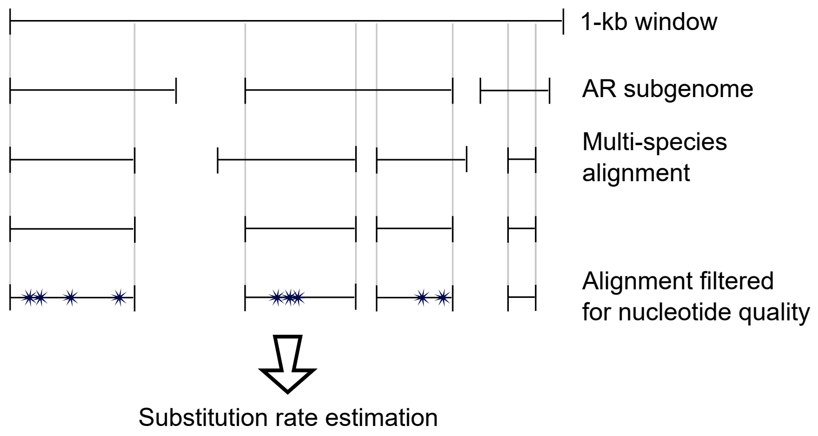


Figure S21: Schematic summary of substitution rate estimation.

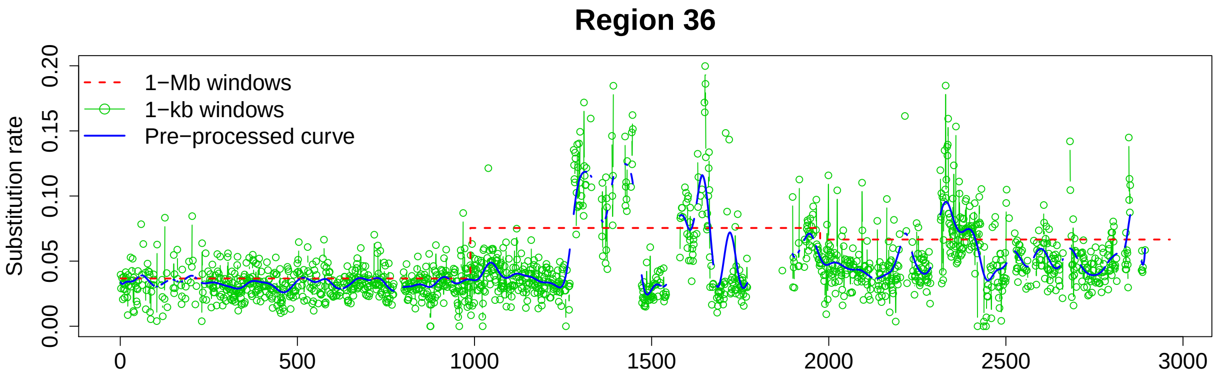


Figure S22: Example of substitution rate curve. The red horizontal lines represent the rates estimated in 1-Mb windows by Kuruppumullage Don et al. (2013), while green points are high-resolution rates estimated in 1-kb windows (only accurate values are shown), and blue curve represents pre-processed data.

by AR neutral subgenome, it can happen that alignments are present only in a portion of this subgenome. In this case rate estimation can be inaccurate, since a very low number of nucleotides corresponding to alignments are compared to compute it.

The resulting 43 substitution rate curves are highly noisy, and contain several missing or inaccurate values, due to the segmented nature of AR subgenome and of the multiple alignments considered to estimate rates (see e.g. Fig. S22). We assume that rates vary continuously in nearby windows along the genome, and we propose to pre-process them with stochastic regression imputation and local smoothing, filling small gaps while retaining large gaps (i.e. long stretches of missing values) for which we do not have enough information. We flag as "inaccurate" all rates estimated using less than 200 nucleotides, and we fill in all gaps comprising at most 5 windows using stochastic weighted regression imputation (see e.g. Enders, 2010). For each sequence of contiguous windows with missing or inaccurate rates (i.e. corresponding to a gap in the curve) we fit a weighted simple linear regression model for the rate – considering 2 neighbor windows on each side of the gaps and weighting each window based on the reliability of its estimate (i.e. employing a weight proportional to

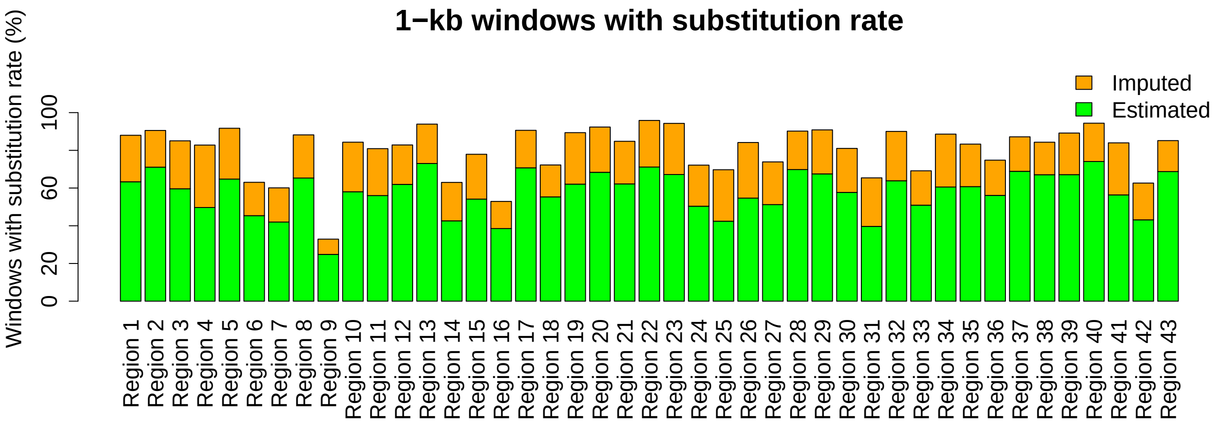


Figure S23: Quality of the substitution rate estimates in the 43 hot regions. Each bar represents the percentage of 1-kb windows with an accurate estimate (green) and the percentage of 1-kb windows with an imputed rate (orange).

the number of nucleotides used to estimate the rate) – and we impute the values according to the model predictions. Next, we add a residual noise to the imputed values, randomly sampling from the residuals of the fitted model with probabilities proportional to their weights. Notably, the vast majority of gaps in our data is quite small ($\leq$5 windows), hence with this imputation pre-processing we are able to fill 92% of the gaps, reducing missing values to 17% of the windows (see Fig. S23). Finally, we employ local polynomials of degree 4 and bandwidth 25 (with Gaussian kernel) on each curve to obtain a smooth functional object and compute the derivative (see Fig. S22).

We employ Sobolev-like distance $d_{0.5}$ to measure similarities between pieces of curves, requiring the intersection between the domain $\tilde{D}_{i,s_{k,i}}$ of each shifted curve and the interval $(0, c_k)$ where the cluster center is defined to be at least as long as 80% of the interval length $c_k$, and at least as long as the minimum motif length $c$ (see Subsection 2.5). We run probKMA for $K = 2, 3, 4, 5$, minimum lengths $c = 40, 50, 60, 70$ and 10 random initializations for each $(K, c)$ pair. Maximum motif length is set to 150. Weighting "fuzziness" parameter is fixed to be $m = 2$, and probKMA iterations are stopped when the global Bhattacharyya distance $BC_{\max} = \max_{k=1,\ldots,K} BC_k$ is less then or equal to $10^{-8}$. Elongation step (see Subsection 2.3) is performed every 5 iterations, when $BC_{\max} \leq 10^{-3}$; each center is elongated up to 50% of its length in either directions, requiring that the relative objective function $J_{m,k}$ increase is less than 5% (i.e. $(J_{m,k,\text{elong}} - J_{m,k})/J_{m,k} < 0.05$). Cleaning step (see Subsection 2.4) is performed every 50 iterations, when $BC_{\max} \leq 10^{-4}$.

ProbKMA produces clusters of varying quality, and candidate motifs of different lengths (see Fig. S24). Candidate motifs that belong to less than 5 curves, as well as the ones with an average cluster silhouette index lower than the $95^{th}$ percentile of all overall average silhouette indices, are filtered out (see Section 3 and Fig. S24(a)). As a result, a total of 54 candidate motifs (out of a total of 560) are retained for post-processing phase.

When computing pairwise distances between candidate motifs (step 1, see Section S2), we require a minimum overlap of 75% of the shortest motif in each pair. Hierarchical clustering dendrogram is cut at height $2R_{all}$, where the global radius $R_{all}$ is set equal to 20 (steps 3-4, see Section S2 and Fig. 4(b)-(c)). Group-specific radii $R_m$, $m = 1, \ldots, M$, and motif selection in each group are done using default values (see Section S2).

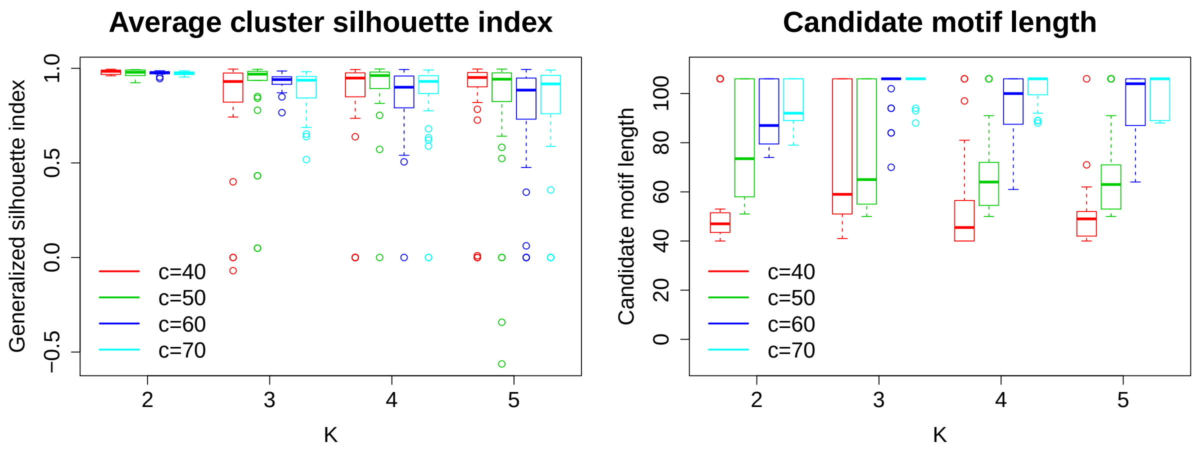


(a) (b)

Figure S24: Candidate motifs produced by probKMA, for $K = 2, 3, 4, 5$ and $c = 40, 50, 60, 70$. (a) Average cluster silhouette index; (b) Candidate motif length.

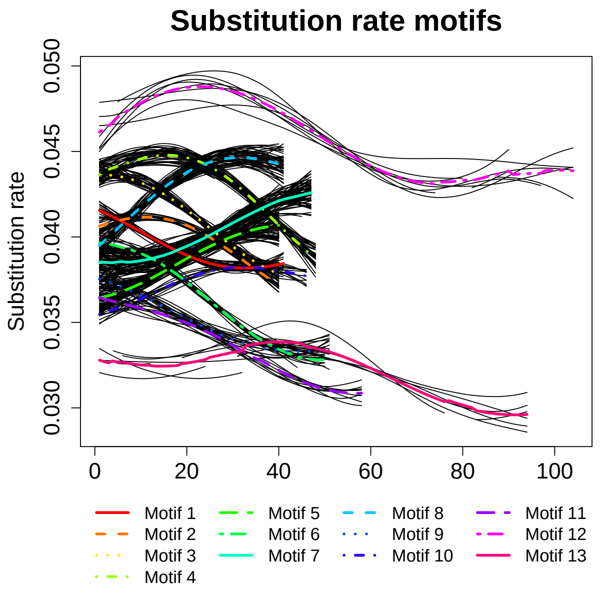


Figure S25: ProbKMA-based functional motif discovery in substitution rate curves. Motifs found plotted in their original scale (colored thick lines) with all occurrences in the data (black solid lines).

Fig. S25 shows motifs found by probKMA-based functional motif discovery and their occurrences in the data, while Fig. S26 shows genomic positions of four of the motifs found. Finally, Table S4 reports the 35 genomic features analyzed (see Fig. 5(b)).

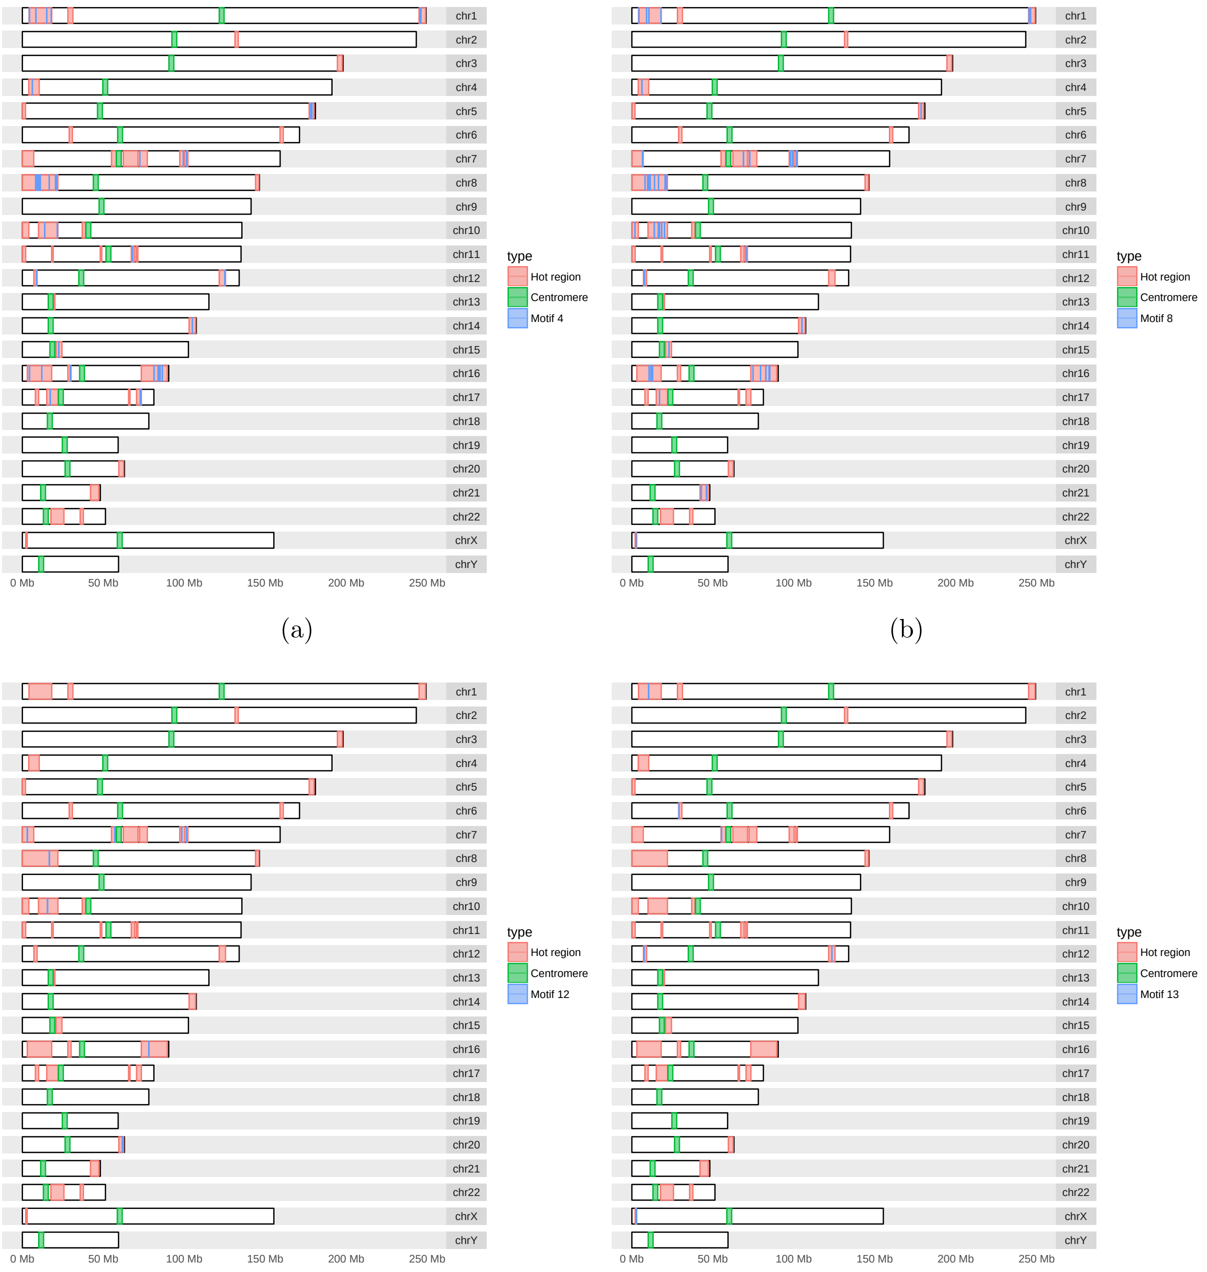


(a) (b) (c) (d)

Figure S26: Genomic positions of motifs found (blue) on hot regions (red). (a) Motif 4; (b) Motif 8; (c) Motif 12; (d) Motif 13.

| | Type | Reference |
|---|---|---|
| **Chromatin structure** | | |
| DNase I hypersensitive sites | Signal | ENCODE (H1-ESC) |
| RNA Polymerase II | Coverage | Barski et al. (2007) |
| CTCF | Signal | ENCODE (H1-ESC) |
| H2AFZ | Signal | ENCODE (H1-ESC) |
| **Transcription regulation** | | |

| | | |
|---|---|---|
| H3K27ac | Signal | ENCODE (H1-ESC) |
| H4K20me1 | Signal | ENCODE (H1-ESC) |
| H3K36me3 | Signal | ENCODE (H1-ESC) |
| H3K4me1 | Signal | ENCODE (H1-ESC) |
| H3K4me2 | Signal | ENCODE (H1-ESC) |
| H3K4me3 | Signal | ENCODE (H1-ESC) |
| H3K79me2 | Signal | ENCODE (H1-ESC) |
| H3K9ac | Signal | ENCODE (H1-ESC) |
| H3K9me3 | Signal | ENCODE (H1-ESC) |
| H3K27me3 | Signal | ENCODE (H1-ESC) |
| **DNA methylation** | | |
| 5-Hydroxymethylcytosine | Count | Szulwach et al. (2011) |
| Sperm hypomethylation | Count | Molaro et al. (2011) |
| **Selection** | | |
| Most conserved elements | Coverage | UCSC Genome Browser |
| CpG islands | Coverage | UCSC Genome Browser |
| Exon | Coverage | UCSC Genome Browser |
| GC content | Percentage | Genome-wide screening |
| **Slippage** | | |
| G-quadruplexes | Coverage | Cer et al. (2011) |
| A-phased repeats | Converage | Cer et al. (2011) |
| Direct repeats | Coverage | Cer et al. (2011) |
| Inverted repeats | Coverage | Cer et al. (2011) |
| Mirror repeats | Coverage | Cer et al. (2011) |
| Z DNA motifs | Coverage | Cer et al. (2011) |
| Mononucleotides | Coverage | Genome-wide screening |
| **Transposition** | | |
| DNA transposons | Coverage | UCSC Genome Browser |
| Alu | Coverage | UCSC Genome Browser |
| MIR | Coverage | UCSC Genome Browser |
| LTR elements | Coverage | UCSC Genome Browser |
| **Gene expression** | | |
| hESC gene expression | Weighted average | UCSC Genome Browser |
| **Replication** | | |
| Replication origins | Count | Besnard et al. (2012) |
| **Recombination** | | |
| Recombination hotspots | Count | Myers et al. (2008) |

Table S4: List of genomic features analyzed (see Fig. 5(b)).

# Supplementary references


Barski, A., S. Cuddapah, K. Cui, T.-Y. Roh, D. E. Schones, Z. Wang, G. Wei, I. Chepelev, and K. Zhao (2007). High-resolution profiling of histone methylations in the human genome. *Cell 129*(4), 823–837.

Besnard, E., A. Babled, L. Lapasset, O. Milhavet, H. Parrinello, C. Dantec, J.-M. Marin, and J.-M. Lemaitre (2012). Unraveling cell type–specific and reprogrammable human replication origin signatures associated with g-quadruplex consensus motifs. *Nature Structural and Molecular Biology 19*(8), 837.

Blankenberg, D., G. V. Kuster, N. Coraor, G. Ananda, R. Lazarus, M. Mangan, A. Nekrutenko, and J. Taylor (2010). Galaxy: a web-based genome analysis tool for experimentalists. *Current Protocols in Molecular Biology Chapter 19*, Unit 19.10 1–21.

Blankenberg, D., J. Taylor, A. Nekrutenko, et al. (2011). Making whole genome multiple alignments usable for biologists. *Bioinformatics 27*(17), 2426–2428.

Cer, R. Z., K. H. Bruce, U. S. Mudunuri, M. Yi, N. Volfovsky, B. T. Luke, A. Bacolla, J. R. Collins, and R. M. Stephens (2011). Non-b db: a database of predicted non-b dna-forming motifs in mammalian genomes. *Nucleic Acids Research 39*(Database Issue), D383–D391.

Enders, C. K. (2010). *Applied missing data analysis*. Guilford Publications.

Goecks, J., A. Nekrutenko, J. Taylor, et al. (2010). Galaxy: a comprehensive approach for supporting accessible, reproducible, and transparent computational research in the life sciences. *Genome Biology 11*(8), R86.

Hardison, R. C., K. M. Roskin, S. Yang, M. Diekhans, W. J. Kent, R. Weber, L. Elnitski, J. Li, M. O'Connor, D. Kolbe, et al. (2003). Covariation in frequencies of substitution, deletion, transposition, and recombination during eutherian evolution. *Genome Research 13*(1), 13–26.

Jukes, T. H. and C. R. Cantor (1969). Evolution of protein molecules. In H. Munro (Ed.), *Mammalian Protein Metabolism*. New York: Academic Press.

Lowe, C. B. and D. Haussler (2012). Mammalian genomes reveal novel exaptations of mobile elements for likely regulatory functions in the human genome. *PLoS One 7*(8), e43128.

Molaro, A., E. Hodges, F. Fang, Q. Song, W. R. McCombie, G. J. Hannon, and A. D. Smith (2011). Sperm methylation profiles reveal features of epigenetic inheritance and evolution in primates. *Cell 146*(6), 1029–1041.

Myers, S., C. Freeman, A. Auton, P. Donnelly, and G. McVean (2008). A common sequence motif associated with recombination hot spots and genome instability in humans. *Nature Genetics 40*(9), 1124.

Smit, A., R. Hubley, and P. Green (2008-2010). RepeatMasker Open-3.0. `http://www.repeatmasker.org`.

Szulwach, K. E., X. Li, Y. Li, C.-X. Song, J. W. Han, S. Kim, S. Namburi, K. Hermetz, J. J. Kim, M. K. Rudd, et al. (2011). Integrating 5-hydroxymethylcytosine into the epigenomic landscape of human embryonic stem cells. *PLoS Genetics 7*(6), e1002154.
